# Supplementary material for: A Khovanov Laplacian and Khovanov Dirac for Knots and Links
Source: arXiv:2411.18841 ancillary file (2024-12-13)
Supplement: Supplementary file 1 [file SupportingInformation_v1.pdf]

# Supporting Information for: Khovanov Laplacian and Khovanov Dirac for Knots and Links

Benjamin Jones †1 and Guo-Wei Wei *1,2,3

[1] Department of Mathematics, Michigan State University, MI, 48824, USA
[2] Department of Electrical and Computer Engineering, Michigan State University, MI 48824, USA
[3] Department of Biochemistry and Molecular Biology, Michigan State University, MI 48824, USA

December 2024

†jones657@msu.edu
*weig@msu.edu

# Contents

**1 Introduction** **3**

**2 Knots of 6 or fewer crossings** **3**

**3 Selected Knots of more than 6 crossings** **28**

# 1 Introduction

This document contains the nonempty spectra of the Khovanov Laplacian for several knots. Since many larger knots have Khovanov Laplacians with hundreds of eigenvalues, we report only the lowest 25 eigenvalues. Eigenvalues are listed in nondecreasing order.

# 2 Knots of 6 or fewer crossings

Table 1: Khovanov Laplacian nonempty spectra for $L = 3_1$. The planar diagram used is PD[X[1, 4, 2, 5], X[3, 6, 4, 1], X[5, 2, 6, 3]].

| Homological Grading $r$ | Quantum Grading $q$ | Spectra $S_L^{r,q}$ |
|---|---|---|
| -3 | -9 | 0 |
| -3 | -7 | 1, 1, 4 |
| -3 | -5 | 2, 2, 5 |
| -3 | -3 | 3 |
| -2 | -7 | 1, 1, 4 |
| -2 | -5 | 0, 2, 2, 5, 6, 6 |
| -2 | -3 | 3, 3, 3 |
| -1 | -5 | 3, 6, 6 |
| -1 | -3 | 3, 3, 6 |
| 0 | -5 | 3 |
| 0 | -3 | 0, 6 |
| 0 | -1 | 0 |

Table 2: Khovanov Laplacian nonempty spectra for $L = 4_1$. The planar diagram used is PD[X[4, 2, 5, 1], X[8, 6, 1, 5], X[6, 3, 7, 4], X[2, 7, 3, 8]].

| Homological Grading $r$ | Quantum Grading $q$ | Spectra $S_L^{r,q}$ |
|---|---|---|
| -2 | -5 | 0 |
| -2 | -3 | 1, 1.43845, 5.56155 |
| -2 | -1 | 2, 3.26795, 6.73205 |
| -2 | 1 | 4 |
| -1 | -3 | 1, 1.43845, 2, 5.56155 |
| -1 | -1 | 0, 2, 2.76393, 3.26795, 6.73205, 7.23607, 8, 8 |
| -1 | 1 | 4, 4, 4, 6 |
| 0 | -3 | 2 |
| 0 | -1 | 0, 2.76393, 4, 4, 6, 7.23607, 8, 8 |
| 0 | 1 | 0, 2.76393, 4, 4, 6, 7.23607, 8, 8 |

| | | |
|---|---|---|
| 0 | 3 | 2 |
| 1 | -1 | 4, 4, 4, 6 |
| 1 | 1 | 0, 2, 2.76393, 3.26795, 6.73205, 7.23607, 8, 8 |
| 1 | 3 | 1, 1.43845, 2, 5.56155 |
| 2 | -1 | 4 |
| 2 | 1 | 2, 3.26795, 6.73205 |
| 2 | 3 | 1, 1.43845, 5.56155 |
| 2 | 5 | 0 |

Table 3: Khovanov Laplacian nonempty spectra for $L = 5_1$. The planar diagram used is PD[X[1, 6, 2, 7], X[3, 8, 4, 9], X[5, 10, 6, 1], X[7, 2, 8, 3], X[9, 4, 10, 5]].

| Homological Grading $r$ | Quantum Grading $q$ | Spectra $S_L^{r,q}$ |
|---|---|---|
| -5 | -15 | 0 |
| -5 | -13 | 0.381966, 0.381966, 2.61803, 2.61803, 4 |
| -5 | -11 | 1.0437, 1.0437, 2, 2.79094, 2.79094, 4.33826, 4.33826, 4.82709, 4.82709, 7 |
| -5 | -9 | 2.0437, 2.0437, 3, 3.79094, 3.79094, 5.33826, 5.33826, 5.82709, 5.82709, 8 |
| -5 | -7 | 3.38197, 3.38197, 5.61803, 5.61803, 7 |
| -5 | -5 | 5 |
| -4 | -13 | 0.381966, 0.381966, 2.61803, 2.61803, 4 |
| -4 | -11 | 0, 1.0437, 1.0437, 2, 2.53327, 2.53327, 2.79094, 2.79094, 3.22252, 3.22252, 4, 4.33826, 4.33826, 4.82709, 4.82709, 5.77748, 5.77748, 6.46673, 6.46673, 7 |
| -4 | -9 | 1.00756, 1.00756, 2.0437, 2.0437, 3, 3.53253, 3.53253, 3.79094, 3.79094, 4, 4, 4, 4, 4, 4, 4, 5.33826, 5.33826, 5.82709, 5.82709, 6, 6, 6, 6, 6 |

| | | |
|---|---|---|
| -4 | -7 | 2.58579, 2.79794, 2.79794, 3.38197, 3.38197, 4.32133, 4.32133, 5.18966, 5.18966, 5.41421, 5.53318, 5.53318, 5.61803, 5.61803, 6, 7, 7.39437, 7.39437, 7.76353, 7.76353 |
| -4 | -5 | 5, 5, 5, 5, 5 |
| -3 | -11 | 0, 2.53327, 2.53327, 3.22252, 3.22252, 4, 5.77748, 5.77748, 6.46673, 6.46673 |
| -3 | -9 | 1.00756, 1.00756, 3, 3, 3, 3, 3.53253, 3.53253, 4, 4, 4, 4, 4, 4, 4, 6, 6, 6, 6, 6, 8, 8, 8, 8, 8 |
| -3 | -7 | 2.58579, 2.79794, 2.79794, 2.93846, 2.93846, 3.49052, 3.49052, 4.32133, 4.32133, 5, 5.18966, 5.18966, 5.28383, 5.28383, 5.41421, 5.49161, 5.49161, 5.53318, 5.53318, 6, 7.39437, 7.39437, 7.76353, 7.76353, 8 |
| -3 | -5 | 5, 5, 5, 5, 5, 5, 5, 5, 5, 5 |
| -2 | -9 | 3, 3, 3, 3, 8, 8, 8, 8, 8, 8 |
| -2 | -7 | 0, 2.93846, 2.93846, 3.49052, 3.49052, 5, 5.28383, 5.28383, 5.49161, 5.49161, 8, 8.22565, 8.22565, 8.56993, 8.56993, 9, 10, 10, 10, 10 |
| -2 | -5 | 5, 5, 5, 5, 5, 5, 5, 5, 5, 5 |
| -1 | -7 | 5, 10, 10, 10, 10 |
| -1 | -5 | 5, 5, 5, 5, 10 |
| 0 | -7 | 5 |
| 0 | -5 | 0, 10 |
| 0 | -3 | 0 |

Table 4: Khovanov Laplacian nonempty spectra for $L = 5_2$. The planar diagram used is PD[X[1, 4, 2, 5], X[3, 8, 4, 9], X[5, 10, 6, 1], X[9, 6, 10, 7], X[7, 2, 8, 3]].

| Homological Grading $r$ | Quantum Grading $q$ | Spectra $S_L^{r,q}$ |
|---|---|---|

| | | |
|---|---|---|
| -5 | -13 | 0 |
| -5 | -11 | 1, 1.62772, 7.37228 |
| -5 | -9 | 2, 4.43845, 8.56155 |
| -5 | -7 | 5 |
| -4 | -11 | 1, 1.62772, 3, 3, 7.37228 |
| -4 | -9 | 0, 2, 4, 4, 4.43845, 8.56155, 9, 9, 10, 10 |
| -4 | -7 | 5, 5, 5, 8, 8 |
| -3 | -11 | 3, 3, 3 |
| -3 | -9 | 0, 1.62772, 2.17157, 4, 4, 4, 5, 5, 5, 7, 7.37228, 7.82843, 9, 9, 10, 10 |
| -3 | -7 | 0.604766, 1.13612, 2.47438, 3.69384, 4.52303, 5, 5, 5.89068, 8, 8, 8, 9.33634, 9.34085, 10, 10, 10 |
| -3 | -5 | 3, 3, 6 |
| -2 | -11 | 3 |
| -2 | -9 | 1.62772, 2.17157, 4, 5, 5, 5, 5, 5, 5, 7, 7, 7.37228, 7.82843 |
| -2 | -7 | 0, 0.604766, 1.13612, 2.47438, 2.62772, 2.87623, 3.69384, 4, 4.43845, 4.52303, 5, 5.15644, 5.89068, 6, 8, 8.17276, 8.37228, 8.56155, 8.79456, 9.33634, 9.34085, 10, 10, 10 |
| -2 | -5 | 0, 2, 2.55051, 2.55051, 3, 3, 3, 4, 6, 7, 7.44949, 7.44949, 8 |
| -2 | -3 | 2 |
| -1 | -9 | 5, 5, 5, 5, 7 |
| -1 | -7 | 2.38197, 2.62772, 2.87623, 4, 4.43845, 4.61803, 5, 5.15644, 5.38197, 6, 7.61803, 8.17276, 8.37228, 8.56155, 8.79456 |
| -1 | -5 | 0.740334, 2, 2.55051, 2.55051, 3, 3.17404, 3.38197, 4, 4, 5.61803, 7, 7.44949, 7.44949, 8, 8.08563 |
| -1 | -3 | 0, 2, 2, 2.58579, 5.41421 |
| 0 | -9 | 5 |

| | | |
|---|---|---|
| 0 | -7 | 2.38197, 4.61803, 5.38197, 7.61803 |
| 0 | -5 | 0.740334, 3.17404, 3.38197, 4, 5.61803, 8.08563 |
| 0 | -3 | 0, 2, 2.58579, 5.41421 |
| 0 | -1 | 0 |

Table 5: Khovanov Laplacian nonempty spectra for $L = 6_1$. The planar diagram used is PD[X[1, 4, 2, 5], X[7, 10, 8, 11], X[3, 9, 4, 8], X[9, 3, 10, 2], X[5, 12, 6, 1], X[11, 6, 12, 7]].

| Homological Grading $r$ | Quantum Grading $q$ | Spectra $S_L^{r,q}$ |
|---|---|---|
| -4 | -9 | 0 |
| -4 | -7 | 1, 1.72508, 9.27492 |
| -4 | -5 | 2, 5.55051, 10.4495 |
| -4 | -3 | 6 |
| -3 | -7 | 1, 1.72508, 4, 4, 4, 9.27492 |
| -3 | -5 | 0, 2, 5.17157, 5.17157, 5.17157, 5.55051, 10.4495, 10.8284, 10.8284, 10.8284, 12, 12 |
| -3 | -3 | 6, 6, 6, 10, 10, 10 |
| -2 | -7 | 4, 4, 4, 4, 4, 4 |
| -2 | -5 | 0, 2.171, 2.35342, 2.96624, 3.52956, 4, 5.06982, 5.17157, 5.17157, 5.17157, 5.20425, 5.5475, 6, 6, 6, 6, 8, 8.40112, 8.59537, 9.1508, 9.39182, 9.6191, 10.8284, 10.8284, 10.8284 |
| -2 | -3 | 1.04584, 2.025, 2.10371, 3.09538, 3.84753, 4.44146, 5.20948, 5.35554, 6, 6, 6.09409, 7.46182, 7.81495, 7.95148, 9.54489, 9.76742, 10, 10, 10, 10, 11.4118, 11.4121, 11.4175, 12, 12 |
| -2 | -1 | 4, 4, 4, 8, 8, 8 |
| -1 | -7 | 4, 4, 4, 4 |
| -1 | -5 | 2, 2.171, 2.35342, 2.96624, 3.52956, 3.55051, 4, 4, 5.06982, 5.20425, 5.26795, 5.5475, 6, 6, 6, 6, 6, 6, 6, 6, 6, 6, 8, 8, 8 |

| | | |
|---|---|---|
| -1 | -3 | 0, 0.627607, 1.04584, 2.025, 2.10371, 2.55656, 2.57342, 3.08822, 3.09538, 3.21683, 3.43416, 3.48547, 3.71239, 3.84753, 4.44146, 4.65331, 4.86927, 5.20948, 5.22785, 5.2534, 5.35554, 6, 6.09409, 6.19071, 6.31993 |
| -1 | -1 | 0, 1.38368, 2.03884, 3, 3.1101, 3.46806, 3.62772, 3.62772, 3.62772, 4, 4, 4, 4.17095, 4.8221, 5, 5, 6, 6.0432, 7.00609, 8, 8, 8, 8.57779, 8.57849, 9.21172 |
| -1 | 1 | 2, 4, 4, 6 |
| 0 | -7 | 4 |
| 0 | -5 | 2, 3.55051, 4, 5.26795, 6, 6, 6, 6, 6, 6, 6, 6, 6, 6, 8, 8, 8, 8.44949, 8.73205 |
| 0 | -3 | 0.627607, 2.55656, 2.57342, 3.01132, 3.08822, 3.17027, 3.21683, 3.28727, 3.43416, 3.48547, 3.71239, 4.65331, 4.86927, 5.0846, 5.09679, 5.2269, 5.22785, 5.2534, 5.86856, 6, 6.19071, 6.31993, 6.32409, 6.33114, 6.48467 |
| 0 | -1 | 0, 1.1323, 1.18175, 1.38368, 2.03884, 3, 3.1101, 3.29844, 3.46806, 3.62772, 3.62772, 3.62772, 3.7498, 3.93986, 4.17095, 4.38657, 4.41076, 4.45247, 4.61099, 4.8221, 5, 5, 5, 5, 5 |
| 0 | 1 | 0, 0, 2, 2.29072, 2.62772, 2.93356, 3.43845, 4, 4, 4, 4, 4.77781, 4.80606, 6, 6.65222, 6.90321, 7.56155, 7.6364, 8.37228 |
| 0 | 3 | 2 |
| 1 | -5 | 6, 6, 6, 6, 6, 8 |

| | | |
|---|---|---|
| 1 | -3 | 3.01132, 3.17027, 3.28727, 3.58579, 4.43845, 5.0846, 5.09679, 5.2269, 5.86856, 6.33114, 6.41421, 6.48467, 6.64955, 6.82447, 7, 7.19394, 7.26673, 8, 8.56155, 8.89711, 9, 9.35541, 9.542, 9.70928 |
| 1 | -1 | 1.1323, 1.18175, 2.13455, 2.419, 3.29844, 3.7498, 3.82003, 3.93986, 4.30229, 4.38657, 4.39539, 4.41076, 4.45247, 4.61099, 5, 5, 5, 5.36953, 5.89748, 6, 6.53994, 6.5553, 7, 7, 7.10112 |
| 1 | 1 | 0, 1.05559, 1.27838, 2.26652, 2.29072, 2.62772, 2.81508, 2.93356, 3.43845, 3.89432, 4, 4, 4.55717, 4.77781, 4.80606, 4.82275, 6.10426, 6.57216, 6.65222, 6.90321, 7.56155, 7.6364, 8.37228, 8.63377 |
| 1 | 3 | 0.381966, 0.471082, 2, 2.61803, 3.16745, 5.36147 |
| 2 | -5 | 6 |
| 2 | -3 | 3.58579, 4.43845, 6.41421, 7, 8.56155 |
| 2 | -1 | 2.13455, 2.419, 3.82003, 4.30229, 4.39539, 5.89748, 6.53994, 7.20372, 7.57258, 9.71503 |
| 2 | 1 | 1.05559, 1.27838, 2.26652, 2.81508, 3.89432, 4.55717, 4.82275, 6.10426, 6.57216, 8.63377 |
| 2 | 3 | 0.381966, 0.471082, 2.61803, 3.16745, 5.36147 |
| 2 | 5 | 0 |

Table 6: Khovanov Laplacian nonempty spectra for $L = 6_2$. The planar diagram used is PD[X[1, 4, 2, 5], X[5, 10, 6, 11], X[3, 9, 4, 8], X[9, 3, 10, 2], X[7, 12, 8, 1], X[11, 6, 12, 7]].

| Homological Grading $r$ | Quantum Grading $q$ | Spectra $S_L^{r,q}$ |
|---|---|---|
| -4 | -11 | 0 |
| -4 | -9 | 0.381966, 1.13919, 2.61803, 2.7459, 5.11491 |
| -4 | -7 | 1.43632, 1.58579, 3, 3.27509, 3.38197, 4.41421, 5.10517, 5.61803, 5.95959, 8.22382 |
| -4 | -5 | 2.49881, 3.06815, 3.95907, 4.48236, 4.8685, 5.51764, 6.40757, 6.9021, 6.93185, 9.36394 |
| -4 | -3 | 4, 4.82991, 6, 6.68889, 8.48119 |
| -4 | -1 | 6 |
| -3 | -9 | 0, 0.381966, 1.13919, 2.61803, 2.7459, 5.11491 |
| -3 | -7 | 0, 1.12373, 1.43632, 1.58579, 1.80394, 2.43457, 2.77817, 3, 3.27509, 3.31525, 3.33134, 3.38197, 3.83581, 4.13905, 4.41421, 5.10517, 5.61803, 5.95959, 6.89062, 7.26874, 7.55042, 7.67876, 7.8496, 8.22382 |
| -3 | -5 | 0.90343, 1.91764, 2.49881, 2.67927, 2.72976, 3.06815, 3.3872, 3.85157, 3.95907, 4, 4.02861, 4.15184, 4.26795, 4.48236, 4.65154, 4.70664, 4.8685, 5, 5.51764, 5.61135, 6.14565, 6.40757, 6.50129, 6.9021, 6.93185 |
| -3 | -3 | 2.6699, 3.68656, 3.87037, 4, 4.31963, 4.43541, 4.82991, 5, 5.08734, 5.64094, 6, 6, 6.09119, 6.29126, 6.53532, 6.68889, 6.98284, 7.12946, 8.48119, 8.89793, 9.05422, 9.31031, 9.46237, 9.53494 |
| -3 | -1 | 6, 6, 6, 6, 6, 6 |

| | | |
|---|---|---|
| -2 | -7 | 0, 1.12373, 1.80394, 2.43457, 2.77817, 3, 3.31525, 3.33134, 3.83581, 4.13905, 6.89062, 7.26874, 7.55042, 7.67876, 7.8496 |
| -2 | -5 | 0, 0.90343, 1.91764, 2.67927, 2.72976, 3, 3.29844, 3.3872, 3.45862, 3.45862, 3.80742, 3.80742, 3.85157, 4, 4, 4.02861, 4.15184, 4.26795, 4.65154, 4.70664, 5, 5.26795, 5.61135, 6.14565, 6.50129 |
| -2 | -3 | 1.78701, 2.6699, 2.77057, 2.81985, 3.68656, 3.82226, 3.87037, 4.18373, 4.26058, 4.31963, 4.43541, 4.75316, 5, 5.08734, 5.23549, 5.55051, 5.64094, 5.80327, 6, 6.09119, 6.2189, 6.26512, 6.29126, 6.53532, 6.69663 |
| -2 | -1 | 6, 6, 6, 6, 6, 6, 6, 6, 6, 6, 6, 6, 6, 6, 9 |
| -1 | -7 | 3 |
| -1 | -5 | 0, 3, 3.29844, 3.45862, 3.45862, 3.80742, 3.80742, 4, 4, 4, 4, 5.26795, 7, 8.73205, 9.19258, 9.19258, 9.54138, 9.54138, 9.70156, 10, 10, 10, 10 |
| -1 | -3 | 0, 0.622878, 1.12462, 1.78701, 2.77057, 2.81909, 2.81985, 3.82226, 4.18373, 4.26058, 4.75316, 4.76027, 5.17157, 5.23549, 5.55051, 5.75944, 5.80327, 6.2189, 6.26512, 6.69663, 6.86994, 7.12646, 7.42216, 8, 9.82297 |
| -1 | -1 | 1.59488, 2.18541, 4.09637, 6, 6, 6, 6, 6, 6, 6, 6, 6, 6, 6, 6, 6, 6, 9, 9, 9.40512, 9.71821, 10 |
| -1 | 1 | 3 |

| | | |
|---|---|---|
| 0 | -5 | 4, 4, 4, 7 |
| 0 | -3 | 0, 0.622878, 1.12462, 2.81909, 4.76027, 5.17157, 5.75944, 6, 6, 6.86994, 8, 9, 9, 9.82297, 10.8284, 11.1049, 11.1159, 12, 12, 12, 12, 12, 12 |
| 0 | -1 | 0, 0, 1.59488, 2.18541, 2.87689, 4.09637, 4.1459, 4.1459, 6, 6, 6, 6, 6, 6, 9, 9.40512, 9.71821, 10, 10.8541, 10.8541, 11.1231, 12, 12 |
| 0 | 1 | 2, 3, 3, 3 |
| 1 | -3 | 6, 6, 6, 8, 9, 9 |
| 1 | -1 | 0, 2.79809, 2.87689, 4.1459, 4.1459, 5.08882, 10.1131, 10.8541, 10.8541, 11.1231, 12, 12 |
| 1 | 1 | 1.1944, 2, 2.38677, 3, 3, 8.41883 |
| 2 | -3 | 6 |
| 2 | -1 | 2.79809, 5.08882, 10.1131 |
| 2 | 1 | 1.1944, 2.38677, 8.41883 |
| 2 | 3 | 0 |

Table 7: Khovanov Laplacian nonempty spectra for $L = 6_3$. The planar diagram used is PD[X[4, 2, 5, 1], X[8, 4, 9, 3], X[12, 9, 1, 10], X[10, 5, 11, 6], X[6, 11, 7, 12], X[2, 8, 3, 7]].

| Homological Grading $r$ | Quantum Grading $q$ | Spectra $S_L^{r,q}$ |
|---|---|---|
| -3 | -7 | 0 |
| -3 | -5 | 0.789816, 2, 2.73929, 6.4709 |
| -3 | -3 | 1.97131, 3.29567, 3.85542, 5.10659, 6.48042, 9.2906 |
| -3 | -1 | 3.72693, 5, 6.14044, 9.13264 |
| -3 | 1 | 6 |
| -2 | -5 | 0, 0.789816, 2, 2, 2.73929, 6.4709 |
| -2 | -3 | 0, 1.97131, 2.1459, 2.70742, 3, 3.29567, 3.29844, 3.35425, 3.85542, 4, 5.10659, 6.48042, 8.64575, 8.72165, 8.8541, 9.2906, 9.57093, 9.70156 |

| | | |
|---|---|---|
| -2 | -1 | 1.78587, 2.76468, 3.72693, 3.74475, 4.48622, 4.72693, 5, 5.23682, 6.14044, 6.21839, 6.67426, 7.14044, 9.13264, 9.89283, 10.1281, 10.1326, 10.5127, 10.5554 |
| -2 | 1 | 6, 6, 6, 6, 6, 8 |
| -1 | -5 | 2 |
| -1 | -3 | 0, 2.1459, 2.70742, 3, 3, 3, 3.29844, 3.35425, 3.43845, 4, 4, 4, 7.56155, 8.64575, 8.72165, 8.8541, 9.57093, 9.70156 |
| -1 | -1 | 0, 0.645488, 1.55245, 1.78587, 2.73836, 2.76468, 3.74475, 4.11116, 4.1459, 4.48622, 4.72693, 5.17157, 5.17157, 5.23682, 5.26356, 6.21839, 6.67426, 7.14044, 7.62347, 9.47349, 9.89283, 10.1281, 10.1326, 10.5127, 10.5554 |
| -1 | 1 | 1.94763, 3.01264, 5.13962, 6, 6, 6, 6, 6, 6, 6, 6, 8, 8, 8.44605, 9, 9.45406, 10, 10 |
| -1 | 3 | 4 |
| 0 | -3 | 3, 3, 3.43845, 4, 4, 4, 7.56155 |
| 0 | -1 | 0, 0, 0.645488, 1.55245, 1.94763, 2.73836, 3.01264, 4.11116, 4.1459, 5.13962, 5.17157, 5.17157, 5.26356, 6, 6, 6, 6, 7.62347, 8, 8.44605, 9, 9.45406, 9.47349, 10, 10 |
| 0 | 1 | 0, 0, 0.645488, 1.55245, 1.94763, 2.73836, 3.01264, 4.11116, 4.1459, 5.13962, 5.17157, 5.17157, 5.26356, 6, 6, 6, 6, 7.62347, 8, 8.44605, 9, 9.45406, 9.47349, 10, 10 |
| 0 | 3 | 3, 3, 3.43845, 4, 4, 4, 7.56155 |
| 1 | -3 | 4 |

| | | |
|---|---|---|
| 1 | -1 | 1.94763, 3.01264, 5.13962, 6, 6, 6, 6, 6, 6, 6, 6, 8, 8, 8.44605, 9, 9.45406, 10, 10 |
| 1 | 1 | 0, 0.645488, 1.55245, 1.78587, 2.73836, 2.76468, 3.74475, 4.11116, 4.1459, 4.48622, 4.72693, 5.17157, 5.17157, 5.23682, 5.26356, 6.21839, 6.67426, 7.14044, 7.62347, 9.47349, 9.89283, 10.1281, 10.1326, 10.5127, 10.5554 |
| 1 | 3 | 0, 2.1459, 2.70742, 3, 3, 3, 3.29844, 3.35425, 3.43845, 4, 4, 4, 7.56155, 8.64575, 8.72165, 8.8541, 9.57093, 9.70156 |
| 1 | 5 | 2 |
| 2 | -1 | 6, 6, 6, 6, 6, 8 |
| 2 | 1 | 1.78587, 2.76468, 3.72693, 3.74475, 4.48622, 4.72693, 5, 5.23682, 6.14044, 6.21839, 6.67426, 7.14044, 9.13264, 9.89283, 10.1281, 10.1326, 10.5127, 10.5554 |
| 2 | 3 | 0, 1.97131, 2.1459, 2.70742, 3, 3.29567, 3.29844, 3.35425, 3.85542, 4, 5.10659, 6.48042, 8.64575, 8.72165, 8.8541, 9.2906, 9.57093, 9.70156 |
| 2 | 5 | 0, 0.789816, 2, 2, 2.73929, 6.4709 |
| 3 | -1 | 6 |
| 3 | 1 | 3.72693, 5, 6.14044, 9.13264 |
| 3 | 3 | 1.97131, 3.29567, 3.85542, 5.10659, 6.48042, 9.2906 |
| 3 | 5 | 0.789816, 2, 2.73929, 6.4709 |
| 3 | 7 | 0 |

| homological grading $r$ | quantum grading $q$ | Spectra $S_L^{r,q}$ |
|---|---|---|
| -3 | -9 | 0 |
| -3 | -7 | 1, 1, 4 |

| | | |
|---|---|---|
| -3 | -5 | 2, 2, 5 |
| -3 | -3 | 3 |
| -2 | -7 | 1, 1, 4 |
| -2 | -5 | 0, 2, 2, 5, 6, 6 |
| -2 | -3 | 3, 3, 3 |
| -1 | -5 | 3, 6, 6 |
| -1 | -3 | 3, 3, 6 |
| 0 | -5 | 3 |
| 0 | -3 | 0, 6 |
| 0 | -1 | 0 |

Table 8: Combinatorial Laplacian nonempty spectra for $3_1$, the right handed trefoil.

| homological grading $r$ | quantum grading $q$ | Spectra $S_L^{r,q}$ |
|---|---|---|
| -2 | -5 | 0 |
| -2 | -3 | 1, 1.43845, 5.56155 |
| -2 | -1 | 2, 3.26795, 6.73205 |
| -2 | 1 | 4 |
| -1 | -3 | 1, 1.43845, 2, 5.56155 |
| -1 | -1 | 0, 2, 2.76393, 3.26795, 6.73205, 7.23607, 8, 8 |
| -1 | 1 | 4, 4, 4, 6 |
| 0 | -3 | 2 |
| 0 | -1 | 0, 2.76393, 4, 4, 6, 7.23607, 8, 8 |
| 0 | 1 | 0, 2.76393, 4, 4, 6, 7.23607, 8, 8 |
| 0 | 3 | 2 |
| 1 | -1 | 4, 4, 4, 6 |
| 1 | 1 | 0, 2, 2.76393, 3.26795, 6.73205, 7.23607, 8, 8 |
| 1 | 3 | 1, 1.43845, 2, 5.56155 |
| 2 | -1 | 4 |
| 2 | 1 | 2, 3.26795, 6.73205 |
| 2 | 3 | 1, 1.43845, 5.56155 |
| 2 | 5 | 0 |

Table 9: Combinatorial Laplacian nonempty spectra for $4_1$, the .

| homological grading $r$ | quantum grading $q$ | Spectra $S_L^{r,q}$ |
|---|---|---|
| -5 | -15 | 0 |

| | | |
|---|---|---|
| -5 | -13 | 0.381966, 0.381966, 2.61803, 2.61803, 4 |
| -5 | -11 | 1.0437, 1.0437, 2, 2.79094, 2.79094, 4.33826, 4.33826, 4.82709, 4.82709, 7 |
| -5 | -9 | 2.0437, 2.0437, 3, 3.79094, 3.79094, 5.33826, 5.33826, 5.82709, 5.82709, 8 |
| -5 | -7 | 3.38197, 3.38197, 5.61803, 5.61803, 7 |
| -5 | -5 | 5 |
| -4 | -13 | 0.381966, 0.381966, 2.61803, 2.61803, 4 |
| -4 | -11 | 0, 1.0437, 1.0437, 2, 2.53327, 2.53327, 2.79094, 2.79094, 3.22252, 3.22252, 4, 4.33826, 4.33826, 4.82709, 4.82709, 5.77748, 5.77748, 6.46673, 6.46673, 7 |
| -4 | -9 | 1.00756, 1.00756, 2.0437, 2.0437, 3, 3.53253, 3.53253, 3.79094, 3.79094, 4, 4, 4, 4, 4, 4, 4, 5.33826, 5.33826, 5.82709, 5.82709, 6, 6, 6, 6, 6, 8, 8.0855, 8.0855, 8.37441, 8.37441 |
| -4 | -7 | 2.58579, 2.79794, 2.79794, 3.38197, 3.38197, 4.32133, 4.32133, 5.18966, 5.18966, 5.41421, 5.53318, 5.53318, 5.61803, 5.61803, 6, 7, 7.39437, 7.39437, 7.76353, 7.76353 |
| -4 | -5 | 5, 5, 5, 5, 5 |
| -3 | -11 | 0, 2.53327, 2.53327, 3.22252, 3.22252, 4, 5.77748, 5.77748, 6.46673, 6.46673 |
| -3 | -9 | 1.00756, 1.00756, 3, 3, 3, 3, 3.53253, 3.53253, 4, 4, 4, 4, 4, 4, 4, 6, 6, 6, 6, 6, 8, 8, 8, 8, 8, 8, 8.0855, 8.0855, 8.37441, 8.37441 |

| | | |
|---|---|---|
| -3 | -7 | 2.58579, 2.79794, 2.79794, 2.93846, 2.93846, 3.49052, 3.49052, 4.32133, 4.32133, 5, 5.18966, 5.18966, 5.28383, 5.28383, 5.41421, 5.49161, 5.49161, 5.53318, 5.53318, 6, 7.39437, 7.39437, 7.76353, 7.76353, 8, 8.22565, 8.22565, 8.56993, 8.56993, 9 |
| -3 | -5 | 5, 5, 5, 5, 5, 5, 5, 5, 5, 5 |
| -2 | -9 | 3, 3, 3, 3, 8, 8, 8, 8, 8, 8 |
| -2 | -7 | 0, 2.93846, 2.93846, 3.49052, 3.49052, 5, 5.28383, 5.28383, 5.49161, 5.49161, 8, 8.22565, 8.22565, 8.56993, 8.56993, 9, 10, 10, 10, 10 |
| -2 | -5 | 5, 5, 5, 5, 5, 5, 5, 5, 5, 5 |
| -1 | -7 | 5, 10, 10, 10, 10 |
| -1 | -5 | 5, 5, 5, 5, 10 |
| 0 | -7 | 5 |
| 0 | -5 | 0, 10 |
| 0 | -3 | 0 |

Table 10: Combinatorial Laplacian nonempty spectra for $5_1$, the .

| homological grading $r$ | quantum grading $q$ | Spectra $S_L^{r,q}$ |
|---|---|---|
| -5 | -13 | 0 |
| -5 | -11 | 1, 1.62772, 7.37228 |
| -5 | -9 | 2, 4.43845, 8.56155 |
| -5 | -7 | 5 |
| -4 | -11 | 1, 1.62772, 3, 3, 7.37228 |
| -4 | -9 | 0, 2, 4, 4, 4.43845, 8.56155, 9, 9, 10, 10 |
| -4 | -7 | 5, 5, 5, 8, 8 |
| -3 | -11 | 3, 3, 3 |
| -3 | -9 | 0, 1.62772, 2.17157, 4, 4, 4, 5, 5, 5, 7, 7.37228, 7.82843, 9, 9, 10, 10 |

| | | |
|---|---|---|
| -3 | -7 | 0.604766, 1.13612, 2.47438, 3.69384, 4.52303, 5, 5, 5.89068, 8, 8, 8, 9.33634, 9.34085, 10, 10, 10 |
| -3 | -5 | 3, 3, 6 |
| -2 | -11 | 3 |
| -2 | -9 | 1.62772, 2.17157, 4, 5, 5, 5, 5, 5, 5, 7, 7, 7.37228, 7.82843 |
| -2 | -7 | 0, 0.604766, 1.13612, 2.47438, 2.62772, 2.87623, 3.69384, 4, 4.43845, 4.52303, 5, 5.15644, 5.89068, 6, 8, 8.17276, 8.37228, 8.56155, 8.79456, 9.33634, 9.34085, 10, 10, 10 |
| -2 | -5 | 0, 2, 2.55051, 2.55051, 3, 3, 3, 4, 6, 7, 7.44949, 7.44949, 8 |
| -2 | -3 | 2 |
| -1 | -9 | 5, 5, 5, 5, 7 |
| -1 | -7 | 2.38197, 2.62772, 2.87623, 4, 4.43845, 4.61803, 5, 5.15644, 5.38197, 6, 7.61803, 8.17276, 8.37228, 8.56155, 8.79456 |
| -1 | -5 | 0.740334, 2, 2.55051, 2.55051, 3, 3.17404, 3.38197, 4, 4, 5.61803, 7, 7.44949, 7.44949, 8, 8.08563 |
| -1 | -3 | 0, 2, 2, 2.58579, 5.41421 |
| 0 | -9 | 5 |
| 0 | -7 | 2.38197, 4.61803, 5.38197, 7.61803 |
| 0 | -5 | 0.740334, 3.17404, 3.38197, 4, 5.61803, 8.08563 |
| 0 | -3 | 0, 2, 2.58579, 5.41421 |
| 0 | -1 | 0 |

Table 11: Combinatorial Laplacian nonempty spectra for $5_2$, the .

| homological grading $r$ | quantum grading $q$ | Spectra $S_L^{r,q}$ |
|---|---|---|
| -4 | -9 | 0 |
| -4 | -7 | 1, 1.72508, 9.27492 |
| -4 | -5 | 2, 5.55051, 10.4495 |

| | | |
|---|---|---|
| -4 | -3 | 6 |
| -3 | -7 | 1, 1.72508, 4, 4, 4, 9.27492 |
| -3 | -5 | 0, 2, 5.17157, 5.17157, 5.17157, 5.55051, 10.4495, 10.8284, 10.8284, 10.8284, 12, 12 |
| -3 | -3 | 6, 6, 6, 10, 10, 10 |
| -2 | -7 | 4, 4, 4, 4, 4, 4 |
| -2 | -5 | 0, 2.171, 2.35342, 2.96624, 3.52956, 4, 5.06982, 5.17157, 5.17157, 5.17157, 5.20425, 5.5475, 6, 6, 6, 6, 8, 8.40112, 8.59537, 9.1508, 9.39182, 9.6191, 10.8284, 10.8284, 10.8284, 12, 12 |
| -2 | -3 | 1.04584, 2.025, 2.10371, 3.09538, 3.84753, 4.44146, 5.20948, 5.35554, 6, 6, 6.09409, 7.46182, 7.81495, 7.95148, 9.54489, 9.76742, 10, 10, 10, 10, 11.4118, 11.4121, 11.4175, 12, 12, 12, 12 |
| -2 | -1 | 4, 4, 4, 8, 8, 8 |
| -1 | -7 | 4, 4, 4, 4 |
| -1 | -5 | 2, 2.171, 2.35342, 2.96624, 3.52956, 3.55051, 4, 4, 5.06982, 5.20425, 5.26795, 5.5475, 6, 6, 6, 6, 6, 6, 6, 6, 6, 6, 6, 6, 6, 6, 8, 8, 8, 8.40112, 8.44949, 8.59537, 8.73205, 9.1508, 9.39182, 9.6191 |

| | | |
|---|---|---|
| -1 | -3 | 0, 0.627607, 1.04584, 2.025, 2.10371, 2.55656, 2.57342, 3.08822, 3.09538, 3.21683, 3.43416, 3.48547, 3.71239, 3.84753, 4.44146, 4.65331, 4.86927, 5.20948, 5.22785, 5.2534, 5.35554, 6, 6.09409, 6.19071, 6.31993, 6.32409, 6.57624, 6.68626, 6.86009, 7.20327, 7.46182, 7.49011, 7.81495, 7.86912, 7.95148, 8, 9.54489, 9.60194, 9.69911, 9.76742, 9.85561, 10, 10, 10.1545, 10.2777, 10.3001, 10.4482, 10.6182, 10.8263, 11.4118, 11.4121, 11.4175, 12, 12, 12, 12 |
| -1 | -1 | 0, 1.38368, 2.03884, 3, 3.1101, 3.46806, 3.62772, 3.62772, 3.62772, 4, 4, 4, 4.17095, 4.8221, 5, 5, 6, 6.0432, 7.00609, 8, 8, 8, 8.57779, 8.57849, 9.21172, 9.37228, 9.37228, 9.37228, 9.58898, 10, 10, 10 |
| -1 | 1 | 2, 4, 4, 6 |
| 0 | -7 | 4 |
| 0 | -5 | 2, 3.55051, 4, 5.26795, 6, 6, 6, 6, 6, 6, 6, 6, 6, 6, 6, 6, 6, 6, 6, 6, 8, 8, 8, 8.44949, 8.73205 |

| | | |
|---|---|---|
| 0 | -3 | 0.627607, 2.55656, 2.57342, 3.01132, 3.08822, 3.17027, 3.21683, 3.28727, 3.43416, 3.48547, 3.71239, 4.65331, 4.86927, 5.0846, 5.09679, 5.2269, 5.22785, 5.2534, 5.86856, 6, 6.19071, 6.31993, 6.32409, 6.33114, 6.48467, 6.57624, 6.64955, 6.68626, 6.82447, 6.86009, 7.19394, 7.20327, 7.26673, 7.49011, 7.86912, 8, 8, 8.89711, 9, 9.35541, 9.542, 9.60194, 9.69911, 9.70928, 9.85561, 10, 10.1545, 10.2777, 10.3001, 10.4482, 10.6182, 10.8263 |
| 0 | -1 | 0, 1.1323, 1.18175, 1.38368, 2.03884, 3, 3.1101, 3.29844, 3.46806, 3.62772, 3.62772, 3.62772, 3.7498, 3.93986, 4.17095, 4.38657, 4.41076, 4.45247, 4.61099, 4.8221, 5, 5, 5, 5, 5, 5.36953, 6, 6, 6.0432, 6.5553, 7, 7, 7.00609, 7.10112, 7.51903, 7.80092, 7.91467, 8.57779, 8.57849, 9.21172, 9.37228, 9.37228, 9.37228, 9.58898, 9.66712, 9.70156, 9.87642, 10, 10, 10, 10.0825, 10.2489 |
| 0 | 1 | 0, 0, 2, 2.29072, 2.62772, 2.93356, 3.43845, 4, 4, 4, 4, 4.77781, 4.80606, 6, 6.65222, 6.90321, 7.56155, 7.6364, 8.37228 |
| 0 | 3 | 2 |
| 1 | -5 | 6, 6, 6, 6, 6, 8 |

| | | |
|---|---|---|
| 1 | -3 | 3.01132, 3.17027, 3.28727, 3.58579, 4.43845, 5.0846, 5.09679, 5.2269, 5.86856, 6.33114, 6.41421, 6.48467, 6.64955, 6.82447, 7, 7.19394, 7.26673, 8, 8.56155, 8.89711, 9, 9.35541, 9.542, 9.70928 |
| 1 | -1 | 1.1323, 1.18175, 2.13455, 2.419, 3.29844, 3.7498, 3.82003, 3.93986, 4.30229, 4.38657, 4.39539, 4.41076, 4.45247, 4.61099, 5, 5, 5, 5.36953, 5.89748, 6, 6.53994, 6.5553, 7, 7, 7.10112, 7.20372, 7.51903, 7.57258, 7.80092, 7.91467, 9.66712, 9.70156, 9.71503, 9.87642, 10.0825, 10.2489 |
| 1 | 1 | 0, 1.05559, 1.27838, 2.26652, 2.29072, 2.62772, 2.81508, 2.93356, 3.43845, 3.89432, 4, 4, 4.55717, 4.77781, 4.80606, 4.82275, 6.10426, 6.57216, 6.65222, 6.90321, 7.56155, 7.6364, 8.37228, 8.63377 |
| 1 | 3 | 0.381966, 0.471082, 2, 2.61803, 3.16745, 5.36147 |
| 2 | -5 | 6 |
| 2 | -3 | 3.58579, 4.43845, 6.41421, 7, 8.56155 |
| 2 | -1 | 2.13455, 2.419, 3.82003, 4.30229, 4.39539, 5.89748, 6.53994, 7.20372, 7.57258, 9.71503 |
| 2 | 1 | 1.05559, 1.27838, 2.26652, 2.81508, 3.89432, 4.55717, 4.82275, 6.10426, 6.57216, 8.63377 |
| 2 | 3 | 0.381966, 0.471082, 2.61803, 3.16745, 5.36147 |
| 2 | 5 | 0 |

Table 12: Combinatorial Laplacian nonempty spectra for $6_1$, the .

| homological grading $r$ | quantum grading $q$ | Spectra $S_L^{r,q}$ |
|---|---|---|
| -4 | -11 | 0 |
| -4 | -9 | 0.381966, 1.13919, 2.61803, 2.7459, 5.11491 |
| -4 | -7 | 1.43632, 1.58579, 3, 3.27509, 3.38197, 4.41421, 5.10517, 5.61803, 5.95959, 8.22382 |
| -4 | -5 | 2.49881, 3.06815, 3.95907, 4.48236, 4.8685, 5.51764, 6.40757, 6.9021, 6.93185, 9.36394 |
| -4 | -3 | 4, 4.82991, 6, 6.68889, 8.48119 |
| -4 | -1 | 6 |
| -3 | -9 | 0, 0.381966, 1.13919, 2.61803, 2.7459, 5.11491 |
| -3 | -7 | 0, 1.12373, 1.43632, 1.58579, 1.80394, 2.43457, 2.77817, 3, 3.27509, 3.31525, 3.33134, 3.38197, 3.83581, 4.13905, 4.41421, 5.10517, 5.61803, 5.95959, 6.89062, 7.26874, 7.55042, 7.67876, 7.8496, 8.22382 |
| -3 | -5 | 0.90343, 1.91764, 2.49881, 2.67927, 2.72976, 3.06815, 3.3872, 3.85157, 3.95907, 4, 4.02861, 4.15184, 4.26795, 4.48236, 4.65154, 4.70664, 4.8685, 5, 5.51764, 5.61135, 6.14565, 6.40757, 6.50129, 6.9021, 6.93185, 6.93811, 7, 7.60013, 7.73205, 7.77054, 9.34303, 9.35401, 9.36394, 9.62113, 10.0258, 10.0814 |

| | | |
|---|---|---|
| -3 | -3 | 2.6699, 3.68656, 3.87037, 4, 4.31963, 4.43541, 4.82991, 5, 5.08734, 5.64094, 6, 6, 6.09119, 6.29126, 6.53532, 6.68889, 6.98284, 7.12946, 8.48119, 8.89793, 9.05422, 9.31031, 9.46237, 9.53494 |
| -3 | -1 | 6, 6, 6, 6, 6, 6 |
| -2 | -7 | 0, 1.12373, 1.80394, 2.43457, 2.77817, 3, 3.31525, 3.33134, 3.83581, 4.13905, 6.89062, 7.26874, 7.55042, 7.67876, 7.8496 |
| -2 | -5 | 0, 0.90343, 1.91764, 2.67927, 2.72976, 3, 3.29844, 3.3872, 3.45862, 3.45862, 3.80742, 3.80742, 3.85157, 4, 4, 4.02861, 4.15184, 4.26795, 4.65154, 4.70664, 5, 5.26795, 5.61135, 6.14565, 6.50129, 6.93811, 7, 7.60013, 7.73205, 7.77054, 8.73205, 9.19258, 9.19258, 9.34303, 9.35401, 9.54138, 9.54138, 9.62113, 9.70156, 10, 10, 10, 10, 10.0258, 10.0814 |
| -2 | -3 | 1.78701, 2.6699, 2.77057, 2.81985, 3.68656, 3.82226, 3.87037, 4.18373, 4.26058, 4.31963, 4.43541, 4.75316, 5, 5.08734, 5.23549, 5.55051, 5.64094, 5.80327, 6, 6.09119, 6.2189, 6.26512, 6.29126, 6.53532, 6.69663, 6.98284, 7.12646, 7.12946, 7.42216, 8, 8.89793, 9.05422, 9.31031, 9.46237, 9.53494, 9.84768, 9.87214, 9.97498, 10.2408, 10.3709, 10.4469, 10.4495, 10.6187, 10.7007, 10.7621 |

| | | |
|---|---|---|
| -2 | -1 | 6, 6, 6, 6, 6, 6, 6, 6, 6, 6, 6, 6, 6, 6, 9 |
| -1 | -7 | 3 |
| -1 | -5 | 0, 3, 3.29844, 3.45862, 3.45862, 3.80742, 3.80742, 4, 4, 4, 4, 5.26795, 7, 8.73205, 9.19258, 9.19258, 9.54138, 9.54138, 9.70156, 10, 10, 10, 10 |
| -1 | -3 | 0, 0.622878, 1.12462, 1.78701, 2.77057, 2.81909, 2.81985, 3.82226, 4.18373, 4.26058, 4.75316, 4.76027, 5.17157, 5.23549, 5.55051, 5.75944, 5.80327, 6.2189, 6.26512, 6.69663, 6.86994, 7.12646, 7.42216, 8, 9.82297, 9.84768, 9.87214, 9.97498, 10.2408, 10.3709, 10.4469, 10.4495, 10.6187, 10.7007, 10.7621, 10.8284, 11.1049, 11.1159, 12, 12, 12, 12, 12, 12 |
| -1 | -1 | 1.59488, 2.18541, 4.09637, 6, 6, 6, 6, 6, 6, 6, 6, 6, 6, 6, 6, 6, 6, 6, 9, 9, 9.40512, 9.71821, 10 |
| -1 | 1 | 3 |
| 0 | -5 | 4, 4, 4, 7 |
| 0 | -3 | 0, 0.622878, 1.12462, 2.81909, 4.76027, 5.17157, 5.75944, 6, 6, 6.86994, 8, 9, 9, 9.82297, 10.8284, 11.1049, 11.1159, 12, 12, 12, 12, 12, 12 |
| 0 | -1 | 0, 0, 1.59488, 2.18541, 2.87689, 4.09637, 4.1459, 4.1459, 6, 6, 6, 6, 6, 6, 9, 9.40512, 9.71821, 10, 10.8541, 10.8541, 11.1231, 12, 12 |
| 0 | 1 | 2, 3, 3, 3 |
| 1 | -3 | 6, 6, 6, 8, 9, 9 |

| | | |
|---|---|---|
| 1 | -1 | 0, 2.79809, 2.87689, 4.1459, 4.1459, 5.08882, 10.1131, 10.8541, 10.8541, 11.1231, 12, 12 |
| 1 | 1 | 1.1944, 2, 2.38677, 3, 3, 8.41883 |
| 2 | -3 | 6 |
| 2 | -1 | 2.79809, 5.08882, 10.1131 |
| 2 | 1 | 1.1944, 2.38677, 8.41883 |
| 2 | 3 | 0 |

Table 13: Combinatorial Laplacian nonempty spectra for $6_2$, the .

| homological grading $r$ | quantum grading $q$ | Spectra $S_L^{r,q}$ |
|---|---|---|
| -3 | -7 | 0 |
| -3 | -5 | 0.789816, 2, 2.73929, 6.4709 |
| -3 | -3 | 1.97131, 3.29567, 3.85542, 5.10659, 6.48042, 9.2906 |
| -3 | -1 | 3.72693, 5, 6.14044, 9.13264 |
| -3 | 1 | 6 |
| -2 | -5 | 0, 0.789816, 2, 2, 2.73929, 6.4709 |
| -2 | -3 | 0, 1.97131, 2.1459, 2.70742, 3, 3.29567, 3.29844, 3.35425, 3.85542, 4, 5.10659, 6.48042, 8.64575, 8.72165, 8.8541, 9.2906, 9.57093, 9.70156 |
| -2 | -1 | 1.78587, 2.76468, 3.72693, 3.74475, 4.48622, 4.72693, 5, 5.23682, 6.14044, 6.21839, 6.67426, 7.14044, 9.13264, 9.89283, 10.1281, 10.1326, 10.5127, 10.5554 |
| -2 | 1 | 6, 6, 6, 6, 6, 8 |
| -1 | -5 | 2 |
| -1 | -3 | 0, 2.1459, 2.70742, 3, 3, 3, 3.29844, 3.35425, 3.43845, 4, 4, 4, 7.56155, 8.64575, 8.72165, 8.8541, 9.57093, 9.70156 |

| | | |
|---|---|---|
| -1 | -1 | 0, 0.645488, 1.55245, 1.78587, 2.73836, 2.76468, 3.74475, 4.11116, 4.1459, 4.48622, 4.72693, 5.17157, 5.17157, 5.23682, 5.26356, 6.21839, 6.67426, 7.14044, 7.62347, 9.47349, 9.89283, 10.1281, 10.1326, 10.5127, 10.5554, 10.8284, 10.8284, 10.8541, 11.2522, 11.3398, 12, 12, 12, 12 |
| -1 | 1 | 1.94763, 3.01264, 5.13962, 6, 6, 6, 6, 6, 6, 6, 6, 8, 8, 8.44605, 9, 9.45406, 10, 10 |
| -1 | 3 | 4 |
| 0 | -3 | 3, 3, 3.43845, 4, 4, 4, 7.56155 |
| 0 | -1 | 0, 0, 0.645488, 1.55245, 1.94763, 2.73836, 3.01264, 4.11116, 4.1459, 5.13962, 5.17157, 5.17157, 5.26356, 6, 6, 6, 6, 7.62347, 8, 8.44605, 9, 9.45406, 9.47349, 10, 10, 10.8284, 10.8284, 10.8541, 11.2522, 11.3398, 12, 12, 12, 12 |
| 0 | 1 | 0, 0, 0.645488, 1.55245, 1.94763, 2.73836, 3.01264, 4.11116, 4.1459, 5.13962, 5.17157, 5.17157, 5.26356, 6, 6, 6, 6, 7.62347, 8, 8.44605, 9, 9.45406, 9.47349, 10, 10, 10.8284, 10.8284, 10.8541, 11.2522, 11.3398, 12, 12, 12, 12 |
| 0 | 3 | 3, 3, 3.43845, 4, 4, 4, 7.56155 |
| 1 | -3 | 4 |
| 1 | -1 | 1.94763, 3.01264, 5.13962, 6, 6, 6, 6, 6, 6, 6, 6, 8, 8, 8.44605, 9, 9.45406, 10, 10 |

| | | |
|---|---|---|
| 1 | 1 | 0, 0.645488, 1.55245, 1.78587, 2.73836, 2.76468, 3.74475, 4.11116, 4.1459, 4.48622, 4.72693, 5.17157, 5.17157, 5.23682, 5.26356, 6.21839, 6.67426, 7.14044, 7.62347, 9.47349, 9.89283, 10.1281, 10.1326, 10.5127, 10.5554, 10.8284, 10.8284, 10.8541, 11.2522, 11.3398, 12, 12, 12, 12 |
| 1 | 3 | 0, 2.1459, 2.70742, 3, 3, 3, 3.29844, 3.35425, 3.43845, 4, 4, 4, 7.56155, 8.64575, 8.72165, 8.8541, 9.57093, 9.70156 |
| 1 | 5 | 2 |
| 2 | -1 | 6, 6, 6, 6, 6, 8 |
| 2 | 1 | 1.78587, 2.76468, 3.72693, 3.74475, 4.48622, 4.72693, 5, 5.23682, 6.14044, 6.21839, 6.67426, 7.14044, 9.13264, 9.89283, 10.1281, 10.1326, 10.5127, 10.5554 |
| 2 | 3 | 0, 1.97131, 2.1459, 2.70742, 3, 3.29567, 3.29844, 3.35425, 3.85542, 4, 5.10659, 6.48042, 8.64575, 8.72165, 8.8541, 9.2906, 9.57093, 9.70156 |
| 2 | 5 | 0, 0.789816, 2, 2, 2.73929, 6.4709 |
| 3 | -1 | 6 |
| 3 | 1 | 3.72693, 5, 6.14044, 9.13264 |
| 3 | 3 | 1.97131, 3.29567, 3.85542, 5.10659, 6.48042, 9.2906 |
| 3 | 5 | 0.789816, 2, 2.73929, 6.4709 |
| 3 | 7 | 0 |

Table 14: Combinatorial Laplacian nonempty spectra for $6_3$, the .

# 3 Selected Knots of more than 6 crossings

Table 15: Khovanov Laplacian nonempty spectra for $L = 10_43$. The planar diagram used is PD[X[4, 2, 5, 1], X[10, 4, 11, 3], X[14, 8, 15, 7], X[20, 11, 1, 12], X[12, 19, 13, 20], X[8, 14, 9, 13], X[18, 15, 19, 16], X[16, 5, 17, 6], X[6, 17, 7, 18], X[2, 10, 3, 9]].

| Homological Grading $r$ | Quantum Grading $q$ | Spectra $S_L^{r,q}$ |
|---|---|---|
| -5 | -11 | 0 |
| -5 | -9 | 0.757853, 1.37816, 2, 3.17878, 4.47653, 8.20868 |
| -5 | -7 | 2.01363, 2.34168, 3.06221, 3.18939, 3.96482, 4.42171, 4.55596, 5.39532, 5.75657, 6.95739, 7.31553, 8.75752, 9.64385, 10.0704, 12.554 |
| -5 | -5 | 3.44473, 4.04894, 4.21864, 4.78683, 5.23597, 5.76516, 5.85057, 6.37585, 7.00884, 7.47737, 7.74319, 8.21909, 8.65889, 9.5477, 10.0081, 10.8752, 11.1632, 12.3078, 12.4865, 14.7774 |
| -5 | -3 | 5.1432, 5.89602, 6.1751, 7.03048, 7.31801, 7.83293, 8.3694, 9.05383, 9.78476, 10.0355, 10.9301, 11.8812, 12.1099, 13.1804, 15.2592 |
| -5 | -1 | 7.16326, 8.62237, 8.71558, 10.351, 11.3426, 13.8052 |
| -5 | 1 | 10 |
| -4 | -9 | 0, 0, 0.757853, 1.37816, 2, 2, 2, 3.17878, 4.47653, 8.20868 |
| -4 | -7 | 0, 0.86595, 1.34369, 1.55017, 1.80018, 2.01363, 2.14413, 2.34168, 2.38616, 2.78728, 2.84399, 3.02748, 3.06221, 3.18939, 3.29318, 3.4393, 3.51478, 3.67157, 3.81416, 3.96482, 4, 4.29055, 4.42171, 4.55596, 4.70517 |

| | | |
|---|---|---|
| -4 | -5 | 1.17127, 1.70572, 2.10655, 2.76411, 2.91745, 3.06942, 3.42887, 3.44473, 3.52337, 3.85539, 3.92575, 4.00126, 4.04312, 4.04894, 4.14225, 4.21864, 4.37411, 4.48254, 4.65023, 4.69724, 4.76556, 4.78683, 4.81933, 5.09333, 5.11094 |
| -4 | -3 | 2.68881, 3.43835, 3.70221, 4.52251, 4.73942, 4.84859, 5.1432, 5.29929, 5.33057, 5.44921, 5.55629, 5.64353, 5.82008, 5.89602, 5.95713, 6.14498, 6.17208, 6.1751, 6.27488, 6.30335, 6.35471, 6.52729, 6.66762, 6.85099, 6.96477 |
| -4 | -1 | 4.76093, 6.23319, 6.73287, 6.92192, 7.08247, 7.16326, 7.48662, 7.50812, 7.51397, 7.55104, 7.80302, 8.00767, 8.28609, 8.57801, 8.62237, 8.71558, 8.85358, 8.98455, 9.1581, 9.4548, 9.80622, 10.1835, 10.2382, 10.351, 10.3628 |
| -4 | 1 | 10, 10, 10, 10, 10, 10, 10, 10, 12, 12 |
| -3 | -9 | 2, 2 |
| -3 | -7 | 0, 0, 0, 0, 0.86595, 1.34369, 1.55017, 1.80018, 2, 2, 2.14413, 2.38616, 2.4251, 2.60658, 2.78728, 2.84399, 3, 3.02748, 3.15825, 3.24698, 3.29318, 3.4393, 3.51478, 3.67157, 3.81416 |

| | | |
|---|---|---|
| -3 | -5 | 0, 0, 0.361601, 0.547903, 1.14571, 1.17127, 1.19535, 1.43237, 1.70572, 1.98773, 2.0027, 2.01616, 2.10655, 2.29111, 2.76411, 2.78269, 2.91745, 3.06942, 3.07639, 3.20846, 3.28293, 3.30002, 3.42887, 3.43238, 3.4784 |
| -3 | -3 | 1.44441, 1.45723, 1.46928, 1.7279, 1.75388, 2.31122, 2.50156, 2.51375, 2.60245, 2.68881, 2.81605, 3.01864, 3.35061, 3.43835, 3.49778, 3.53756, 3.70221, 3.75378, 3.80048, 3.98692, 4.00065, 4.06425, 4.23029, 4.23496, 4.39436 |
| -3 | -1 | 2.64372, 2.86273, 3.53001, 4.09925, 4.21598, 4.21706, 4.42018, 4.57015, 4.76093, 4.80226, 4.92652, 4.99433, 5.08386, 5.14867, 5.56638, 5.81859, 5.93417, 5.95612, 6.1267, 6.18719, 6.23319, 6.32982, 6.48756, 6.67159, 6.69168 |
| -3 | 1 | 4.55389, 4.76754, 6.246, 6.55067, 7.55051, 7.88265, 8.23233, 8.55542, 9.41218, 9.76154, 10, 10, 10, 10, 10, 10, 10, 10, 10, 10, 10, 10, 10, 10, 10 |
| -3 | 3 | 8, 8 |
| -2 | -7 | 2, 2, 2.4251, 2.60658, 3, 3.15825, 3.24698, 4, 4.72055, 5, 5, 5, 5, 5, 5, 5, 5, 5.76514, 5.80285, 9.93096, 10.3436 |

| | | |
|---|---|---|
| -2 | -5 | 0, 0, 0, 0, 0, 0.361601, 0.547903, 1.14571, 1.19535, 1.43237, 1.74366, 1.98773, 2, 2.0027, 2.01616, 2.0845, 2.29111, 2.78269, 2.98304, 3, 3.03501, 3.07639, 3.1673, 3.20846, 3.28293 |
| -2 | -3 | 0, 0, 0, 0, 0.836199, 0.981738, 0.99143, 1.21314, 1.44441, 1.45723, 1.46747, 1.46928, 1.7006, 1.7279, 1.75388, 2.01816, 2.08574, 2.12693, 2.29323, 2.31122, 2.32416, 2.36666, 2.50156, 2.51375, 2.60245 |
| -2 | -1 | 1.2621, 1.55422, 1.88328, 2.05498, 2.06899, 2.15345, 2.45565, 2.54066, 2.64372, 2.64859, 2.76421, 2.80847, 2.86273, 2.93297, 3.39376, 3.49409, 3.53001, 3.56882, 3.67773, 3.75346, 3.76517, 3.85709, 3.90659, 4.04526, 4.09925 |
| -2 | 1 | 3.58043, 3.78517, 4.09587, 4.14791, 4.18069, 4.36554, 4.47188, 4.53943, 4.55389, 4.7197, 4.73386, 4.76754, 5.12345, 5.39315, 5.39839, 5.79103, 5.82214, 6.05031, 6.2104, 6.246, 6.27225, 6.35649, 6.41742, 6.41934, 6.51231 |
| -2 | 3 | 7, 7, 7.35425, 7.35425, 7.76393, 8, 8, 8, 8, 8, 8, 8, 8, 8, 8, 8, 8, 12.2361, 12.6458, 12.6458, 13 |
| -1 | -7 | 5, 5, 5, 5, 5 |

| | | |
|---|---|---|
| -1 | -5 | 1.74366, 2, 2.0845, 2.98304, 3, 3.00957, 3.03501, 3.1673, 3.55214, 3.88054, 4.06708, 4.10015, 4.23127, 4.25013, 4.36402, 4.4323, 4.5193, 4.71144, 4.83757, 5, 5, 5, 5, 5, 5 |
| -1 | -3 | 0, 0, 0, 0, 0, 0, 0.836199, 0.981738, 0.99143, 1.21314, 1.33922, 1.46747, 1.64657, 1.7006, 1.75522, 1.91849, 1.93682, 2.01816, 2.05211, 2.08574, 2.12375, 2.12693, 2.29323, 2.32416, 2.36666 |
| -1 | -1 | 0, 0, 0, 0, 0, 0.494418, 0.962958, 1.2621, 1.29337, 1.32994, 1.36941, 1.45986, 1.55422, 1.77169, 1.84131, 1.86698, 1.88328, 2.01504, 2.05498, 2.06899, 2.09008, 2.14119, 2.15345, 2.35877, 2.45565 |
| -1 | 1 | 1.28817, 1.81585, 1.93643, 2.11887, 2.19724, 2.26245, 2.42608, 2.5842, 2.7382, 3.00595, 3.1867, 3.33635, 3.35067, 3.55186, 3.58043, 3.72664, 3.78517, 3.79058, 3.80698, 3.8384, 3.85794, 3.862, 3.86657, 3.95425, 3.98639 |
| -1 | 3 | 2.94152, 3.7568, 4.19985, 4.50952, 4.66839, 5.07814, 5.08917, 5.09025, 5.65796, 6, 6.27161, 6.32875, 6.33628, 6.62772, 6.90235, 7, 7, 7, 7, 7, 7, 7, 7, 7.14717, 7.21062 |
| -1 | 5 | 5, 5.76393, 7, 7, 10.2361 |
| 0 | -7 | 5 |

| | | |
|---|---|---|
| 0 | -5 | 3.00957, 4.25013, 4.5193, 5, 5, 5, 5, 5, 5, 5, 5, 5.76393, 5.76393, 5.76393, 5.79498, 5.81453, 5.95976, 7, 7, 7, 7, 7, 7, 7, 7 |
| 0 | -3 | 1.33922, 1.64657, 1.75522, 1.91849, 1.93682, 2.05211, 2.12375, 2.57853, 2.92679, 2.94152, 2.98193, 3.00083, 3.16574, 3.43107, 3.70774, 3.71044, 3.74253, 3.74352, 3.7568, 3.85179, 3.90632, 3.94846, 4.00987, 4.11732, 4.19985 |
| 0 | -1 | 0, 0, 0, 0, 0, 0, 0, 0.494418, 0.962958, 1.28817, 1.29337, 1.32994, 1.36941, 1.45986, 1.77169, 1.84131, 1.86698, 1.88167, 1.93894, 2.01504, 2.09008, 2.11887, 2.14119, 2.19724, 2.35877 |
| 0 | 1 | 0, 0, 0, 0, 0, 0, 0, 0.546972, 0.962958, 1.28817, 1.29337, 1.328, 1.32994, 1.44007, 1.76968, 1.81585, 1.84131, 1.86698, 1.93643, 2.01504, 2.09008, 2.11887, 2.14119, 2.19724, 2.23608 |
| 0 | 3 | 1.33922, 1.63879, 1.64657, 1.75522, 1.99921, 2.05211, 2.12375, 2.57853, 2.92679, 2.94152, 2.98193, 3.00083, 3.43107, 3.59516, 3.70774, 3.71044, 3.73621, 3.74253, 3.74352, 3.7568, 3.85179, 3.90632, 3.94846, 4.11732, 4.19985 |

| | | |
|---|---|---|
| 0 | 5 | 3.00957, 4.25013, 4.5193, 5, 5, 5, 5, 5, 5, 5, 5, 5.76393, 5.76393, 5.76393, 5.79498, 5.81453, 5.95976, 7, 7, 7, 7, 7, 7, 7, 7 |
| 0 | 7 | 5 |
| 1 | -5 | 5, 5.76393, 7, 7, 10.2361 |
| 1 | -3 | 2.94152, 3.7568, 4.19985, 4.50952, 4.66839, 5.07814, 5.08917, 5.09025, 5.65796, 6, 6.27161, 6.32875, 6.33628, 6.62772, 6.90235, 7, 7, 7, 7, 7, 7, 7, 7, 7.14717, 7.21062 |
| 1 | -1 | 1.28817, 1.88167, 1.93894, 2.11887, 2.19724, 2.42608, 2.45482, 2.5842, 2.92419, 3.00595, 3.1867, 3.33635, 3.55186, 3.64959, 3.78167, 3.78517, 3.79058, 3.80698, 3.8384, 3.85794, 3.86657, 3.95425, 3.98639, 4.00114, 4.02671 |
| 1 | 1 | 0, 0, 0, 0, 0, 0.546972, 0.962958, 1.27287, 1.29337, 1.328, 1.32994, 1.44007, 1.55422, 1.76968, 1.84131, 1.86698, 1.88316, 2.01504, 2.05498, 2.09008, 2.12112, 2.14119, 2.15345, 2.23608, 2.35877 |
| 1 | 3 | 0, 0, 0, 0, 0, 0, 0.836199, 0.99143, 1.00278, 1.05805, 1.33922, 1.63879, 1.64657, 1.66199, 1.75522, 1.77496, 1.99921, 2.01816, 2.05211, 2.08574, 2.12375, 2.12693, 2.29323, 2.30184, 2.57853 |

| | | |
|---|---|---|
| 1 | 5 | 1.74366, 2, 2.0845, 2.98304, 3, 3.00957, 3.03501, 3.1673, 3.55214, 3.88054, 4.06708, 4.10015, 4.23127, 4.25013, 4.36402, 4.4323, 4.5193, 4.71144, 4.83757, 5, 5, 5, 5, 5, 5 |
| 1 | 7 | 5, 5, 5, 5, 5 |
| 2 | -3 | 7, 7, 7.35425, 7.35425, 7.76393, 8, 8, 8, 8, 8, 8, 8, 8, 8, 8, 8, 8, 12.2361, 12.6458, 12.6458, 13 |
| 2 | -1 | 3.78167, 3.78517, 4.09587, 4.3183, 4.36554, 4.51866, 4.53943, 4.58933, 4.7197, 4.75911, 4.76754, 4.8523, 4.9394, 5.12345, 5.39315, 5.39839, 5.79103, 6.05031, 6.2104, 6.246, 6.27225, 6.27688, 6.35649, 6.38526, 6.41742 |
| 2 | 1 | 1.27287, 1.55422, 1.88316, 2.05498, 2.12112, 2.15345, 2.45565, 2.48108, 2.67018, 2.76171, 2.84437, 2.86273, 2.94255, 3.39376, 3.49409, 3.50366, 3.56882, 3.60681, 3.67869, 3.75346, 3.76517, 3.85709, 3.90659, 4.09925, 4.1941 |
| 2 | 3 | 0, 0, 0, 0, 0.836199, 0.99143, 1.00278, 1.05805, 1.44125, 1.45723, 1.46983, 1.66199, 1.74722, 1.75149, 1.77496, 2.01816, 2.08574, 2.12693, 2.27942, 2.29323, 2.30184, 2.50156, 2.60245, 2.64944, 2.6558 |
| 2 | 5 | 0, 0, 0, 0, 0, 0.382197, 0.547903, 1.15198, 1.19535, 1.42077, 1.74366, 1.9357, 1.95649, 2, 2.0027, 2.0845, 2.29111, 2.96271, 2.98304, 3, 3.03501, 3.13817, 3.1673, 3.18274, 3.33567 |

| | | |
|---|---|---|
| 2 | 7 | 2, 2, 2.4251, 2.60658, 3, 3.15825, 3.24698, 4, 4.72055, 5, 5, 5, 5, 5, 5, 5, 5, 5.76514, 5.80285, 9.93096, 10.3436 |
| 3 | -3 | 8, 8 |
| 3 | -1 | 4.58933, 4.76754, 6.246, 6.38526, 7.55051, 8, 8.23233, 8.28441, 9.41218, 9.49047, 10, 10, 10, 10, 10, 10, 10, 10, 10, 10, 10, 10, 10, 10, 10, 10, 10, 10, 10, 10, 10, 10 |
| 3 | 1 | 2.67018, 2.86273, 3.50366, 4.09925, 4.21153, 4.21706, 4.41959, 4.56647, 4.76055, 4.80249, 4.90907, 4.99433, 5.07604, 5.13771, 5.7847, 5.8803, 5.93417, 5.95612, 6.01096, 6.02674, 6.18083, 6.18719, 6.36498, 6.55988, 6.60216 |
| 3 | 3 | 1.44125, 1.45723, 1.46983, 1.74722, 1.75149, 2.27942, 2.50156, 2.60245, 2.68787, 2.6973, 2.88149, 3.02818, 3.44815, 3.47307, 3.53756, 3.64969, 3.80048, 3.83813, 3.86772, 4.00263, 4.06425, 4.12497, 4.23029, 4.3464, 4.46612 |
| 3 | 5 | 0, 0, 0.382197, 0.547903, 1.15198, 1.17801, 1.19535, 1.42077, 1.73107, 1.9357, 1.95649, 2.0027, 2.29111, 2.33544, 2.49816, 2.96165, 2.96271, 3.13817, 3.18274, 3.24362, 3.33567, 3.46269, 3.4784, 3.48469, 3.55757 |
| 3 | 7 | 0, 0, 0, 0, 0.868117, 1.29884, 1.54102, 1.9924, 2, 2, 2.12568, 2.4251, 2.49792, 2.60658, 2.67062, 2.84399, 3, 3.15825, 3.24698, 3.25396, 3.32616, 3.51478, 3.53862, 3.89683, 4 |

| | | |
|---|---|---|
| 3 | 9 | 2, 2 |
| 4 | -1 | 10, 10, 10, 10, 10, 10, 10, 10, 12, 12 |
| 4 | 1 | 4.76055, 6.02674, 6.78817, 6.95785, 7.02398, 7.12834, 7.37851, 7.45368, 7.47446, 7.48662, 7.81262, 8.14986, 8.43307, 8.43504, 8.55552, 9, 9, 9.21972, 9.33996, 9.3892, 9.84179, 10.0672, 10.2557, 10.3676, 10.4597 |
| 4 | 3 | 2.68787, 3.64969, 3.83813, 4.46612, 4.47477, 4.83619, 5.01612, 5.09826, 5.3826, 5.39506, 5.49906, 5.55629, 5.75197, 5.84756, 6.06541, 6.11261, 6.13643, 6.18051, 6.22317, 6.34687, 6.35471, 6.52204, 6.63406, 6.75827, 6.8959 |
| 4 | 5 | 1.17801, 1.73107, 2.33544, 2.49816, 2.96165, 3.24362, 3.46269, 3.53262, 3.73836, 3.81657, 3.90819, 3.94195, 3.95629, 4.00126, 4.11842, 4.2577, 4.33205, 4.34027, 4.48003, 4.69651, 4.69724, 4.73897, 4.93644, 5.11094, 5.11671 |
| 4 | 7 | 0, 0.868117, 1.29884, 1.54102, 1.9924, 2.05333, 2.12568, 2.37498, 2.49792, 2.67062, 2.84399, 2.94891, 3.21097, 3.25396, 3.32616, 3.51478, 3.53862, 3.89683, 4, 4, 4.02719, 4.13937, 4.18173, 4.43124, 4.59629 |
| 4 | 9 | 0, 0, 0.787814, 1.35388, 2, 2, 2, 3.43946, 3.90696, 8.51188 |
| 5 | -1 | 10 |

| | | |
|---|---|---|
| 5 | 1 | 7.12834, 8.43307, 9, 10.4597, 11.1308, 13.8482 |
| 5 | 3 | 5.09826, 5.84756, 6.22317, 6.97104, 7.16394, 8.08195, 8.38025, 9.04366, 9.57522, 10.3207, 11.0261, 11.9094, 11.9582, 13.218, 15.1826 |
| 5 | 5 | 3.53262, 3.81657, 4.33205, 4.69651, 5.41561, 5.54033, 5.73941, 6.4937, 7.10488, 7.2839, 7.41181, 8.29931, 8.8864, 9.65998, 10.2435, 10.9268, 11.2541, 12.1712, 12.463, 14.7282 |
| 5 | 7 | 2.05333, 2.37498, 2.94891, 3.21097, 4, 4.18173, 4.9152, 5.16752, 5.57852, 6.27955, 7.82286, 8.82655, 9.93736, 10.1944, 12.5081 |
| 5 | 9 | 0.787814, 1.35388, 2, 3.43946, 3.90696, 8.51188 |
| 5 | 11 | 0 |

Table 16: Khovanov Laplacian nonempty spectra for $L = 10_4 8$. The planar diagram used is PD[X[6, 2, 7, 1], X[8, 4, 9, 3], X[14, 6, 15, 5], X[20, 15, 1, 16], X[16, 9, 17, 10], X[18, 11, 19, 12], X[10, 17, 11, 18], X[12, 19, 13, 20], X[2, 8, 3, 7], X[4, 14, 5, 13]].

| Homological Grading $r$ | Quantum Grading $q$ | Spectra $S_L^{r,q}$ |
|---|---|---|
| -5 | -11 | 0 |
| -5 | -9 | 0.365744, 1.45902, 1.77181, 3.46815, 3.92702, 9.00825 |
| -5 | -7 | 1.23927, 2.40389, 2.56133, 3.13025, 3.56506, 4.07377, 4.70074, 4.79604, 6.11225, 6.39326, 6.81557, 9.21881, 10.7656, 11.4238, 12.8003 |

| | | |
|---|---|---|
| -5 | -5 | 2.56229, 3.64025, 4.08684, 4.5685, 4.6908, 5.44957, 5.83539, 6.17175, 6.49708, 6.92257, 7.66319, 7.96188, 8.84655, 9.39242, 10.1208, 11.8056, 12.3911, 12.8847, 13.1807, 15.3281 |
| -5 | -3 | 4.34992, 5.51387, 5.83133, 6.9689, 7.28739, 7.60294, 8.12995, 8.74736, 8.95293, 10.5827, 11.3141, 11.7876, 13.2829, 13.9471, 15.7008 |
| -5 | -1 | 6.63568, 8.38197, 8.72891, 10.618, 11.3709, 14.2646 |
| -5 | 1 | 10 |
| -4 | -9 | 0, 0.365744, 1.45902, 1.77181, 2, 3, 3, 3.46815, 3.92702, 9.00825 |
| -4 | -7 | 0, 1.00162, 1.13913, 1.23927, 1.79236, 2.17688, 2.40389, 2.52369, 2.56133, 2.94988, 2.98067, 3.13025, 3.5042, 3.5042, 3.56506, 3.68793, 4.07377, 4.10556, 4.10556, 4.24942, 4.51587, 4.57809, 4.70074, 4.79604, 4.81212 |
| -4 | -5 | 0.633667, 1.79828, 2.33442, 2.56229, 2.71363, 2.91467, 3.17349, 3.21656, 3.32172, 3.62795, 3.64025, 3.77224, 3.81482, 4.08684, 4.12392, 4.31029, 4.38098, 4.5685, 4.5901, 4.6281, 4.6281, 4.6908, 4.91022, 4.96647, 5.02315 |

| | | |
|---|---|---|
| -4 | -3 | 1.95722, 2.91186, 4.03707, 4.241, 4.34992, 4.43831, 4.6323, 4.93103, 5.06153, 5.1161, 5.12208, 5.21345, 5.51387, 5.62009, 5.82197, 5.83133, 6.16502, 6.16502, 6.36476, 6.36476, 6.44156, 6.65174, 6.6838, 6.79079, 6.9151 |
| -4 | -1 | 3.85727, 6.1547, 6.3546, 6.56114, 6.63568, 6.6418, 6.68841, 7.71196, 7.9471, 7.9471, 7.95452, 8.10033, 8.38197, 8.5035, 8.72891, 8.78778, 8.81615, 9.60992, 9.67308, 10.1934, 10.3525, 10.477, 10.4788, 10.618, 10.7565 |
| -4 | 1 | 10, 10, 10, 10, 10, 10, 10, 12, 13, 13 |
| -3 | -9 | 2, 3, 3, 3 |
| -3 | -7 | 0, 0, 0, 1.00162, 1.13913, 1.43734, 1.79236, 2.17688, 2.36262, 2.38197, 2.52369, 2.52556, 2.94988, 2.98067, 3.38197, 3.44507, 3.5042, 3.5042, 3.50433, 3.50669, 3.50946, 3.68793, 4.08324, 4.10556, 4.10556 |
| -3 | -5 | 0, 0.309147, 0.540857, 0.570059, 0.633667, 0.785283, 1.42597, 1.78411, 1.79828, 2.01271, 2.03934, 2.30538, 2.33442, 2.5126, 2.64368, 2.7087, 2.71363, 2.89693, 2.91467, 3.17349, 3.20028, 3.21656, 3.21798, 3.25495, 3.32172 |

| | | |
|---|---|---|
| -3 | -3 | 0.953388, 1.46058, 1.48063, 1.51, 1.65148, 1.66948, 1.95722, 2.01667, 2.41578, 2.72474, 2.72881, 2.75407, 2.83862, 2.87834, 2.91186, 3.08104, 3.44584, 3.70648, 3.74013, 3.83935, 3.87859, 3.93968, 3.98449, 4.03707, 4.07637 |
| -3 | -1 | 2.15021, 2.62541, 2.7612, 2.99786, 3.19764, 3.72826, 3.73278, 3.78768, 3.85683, 3.85727, 4.33467, 4.46902, 4.81755, 4.8996, 5.35938, 5.38774, 5.46164, 5.50809, 5.59341, 5.6798, 5.70321, 5.79301, 5.84528, 5.92888, 6.05427 |
| -3 | 1 | 3.78258, 4.38361, 4.83344, 6.26834, 6.34675, 6.38066, 6.65413, 7.9441, 7.94667, 7.95617, 8.60766, 8.92319, 9.10093, 9.4281, 9.45913, 9.52045, 9.96306, 10, 10, 10, 10, 10, 10, 10, 10 |
| -3 | 3 | 8, 8, 8, 11 |
| -2 | -9 | 3 |
| -2 | -7 | 1.43734, 2.36262, 2.38197, 2.52556, 3.38197, 3.38197, 3.44507, 3.50433, 3.50669, 3.50669, 3.50946, 4.08324, 4.61803, 5.32879, 5.61803, 5.61803, 5.69861, 5.85405, 6, 6, 6, 6, 6, 6, 6 |

| | | |
|---|---|---|
| -2 | -5 | 0, 0, 0, 0.309147, 0.540857, 0.570059, 0.785283, 1.42597, 1.78411, 1.79175, 1.84953, 1.87981, 2, 2.01271, 2.03934, 2.30538, 2.5126, 2.52006, 2.64368, 2.7087, 2.75383, 2.84912, 2.89693, 3, 3 |
| -2 | -3 | 0, 0, 0, 0.453482, 0.619709, 0.760019, 0.953388, 1.19307, 1.46058, 1.48063, 1.51, 1.65148, 1.66948, 2.01667, 2.02874, 2.18186, 2.21238, 2.25997, 2.31843, 2.41578, 2.48481, 2.62401, 2.72474, 2.72881, 2.75407 |
| -2 | -1 | 0.774487, 1.25353, 1.37954, 1.44236, 1.68772, 1.89465, 2.02548, 2.15021, 2.32933, 2.44949, 2.61481, 2.62541, 2.7612, 2.99786, 3.03528, 3.07537, 3.19764, 3.20606, 3.27888, 3.38725, 3.63967, 3.72604, 3.72789, 3.72826, 3.73278 |
| -2 | 1 | 2.05915, 2.61566, 3.4694, 3.5619, 3.63922, 3.70018, 3.78258, 3.8938, 4.11366, 4.23279, 4.38361, 4.39249, 4.53143, 4.64818, 4.6713, 4.8286, 4.83344, 4.83676, 4.87623, 5.11708, 5.32263, 5.42701, 5.52253, 5.72768, 5.87478 |
| -2 | 3 | 3.72466, 5.32292, 6.79882, 7, 7.29844, 7.45862, 7.45862, 7.80742, 7.80742, 8, 8, 8, 8, 8, 8, 8, 8, 8, 8, 8, 8, 8, 8, 8, 8 |
| -2 | 5 | 7 |

| | | |
|---|---|---|
| -1 | -7 | 3.38197, 3.50669, 5.61803, 6, 6, 6, 6, 6, 6, 6, 6, 6, 6, 6, 6, 6, 6.28598, 10.2073 |
| -1 | -5 | 1.79175, 1.84953, 1.87981, 2, 2.52006, 2.69926, 2.75383, 2.84912, 3, 3, 3, 3.0665, 3.57108, 3.70086, 3.70366, 3.75048, 3.799, 4.0947, 4.13727, 4.20184, 4.27468, 4.33641, 4.39646, 4.63781, 4.66543 |
| -1 | -3 | 0, 0, 0, 0, 0.453482, 0.619709, 0.760019, 0.909444, 1.19307, 1.24682, 1.81268, 1.87515, 2.02874, 2.18186, 2.21238, 2.25997, 2.26785, 2.31843, 2.45226, 2.48481, 2.62401, 2.68236, 2.69623, 2.79357, 2.83751 |
| -1 | -1 | 0, 0, 0, 0.413802, 0.774487, 1.25353, 1.30081, 1.37954, 1.38541, 1.3955, 1.44236, 1.54809, 1.68772, 1.79789, 1.89465, 2.02548, 2.02685, 2.03425, 2.14812, 2.25233, 2.32933, 2.34345, 2.34722, 2.39965, 2.44949 |
| -1 | 1 | 0.617268, 1.19296, 1.33466, 1.50419, 2.05915, 2.07648, 2.1273, 2.3514, 2.61566, 2.65418, 3.04769, 3.16289, 3.2037, 3.39051, 3.44468, 3.46231, 3.4694, 3.47971, 3.5619, 3.63922, 3.66899, 3.67736, 3.69988, 3.70018, 3.71367 |

| | | |
|---|---|---|
| -1 | 3 | 2, 3.08415, 3.15505, 3.30514, 3.44001, 3.58261, 3.72466, 3.75436, 3.81931, 4.2716, 4.3809, 4.72579, 4.77907, 4.92482, 5.09941, 5.23781, 5.32292, 5.57413, 5.57934, 5.65572, 5.78155, 5.79108, 5.904, 5.98589, 5.99977 |
| -1 | 5 | 4, 5.12373, 5.80394, 6.43457, 6.77817, 7, 7, 7, 7, 7, 7.31525, 7.33134, 7.83581, 8.13905, 10.8906, 11.2687, 11.5504, 11.6788, 11.8496 |
| 0 | -7 | 6, 6, 6, 6, 6, 6 |
| 0 | -5 | 2.69926, 3, 3.70366, 3.75048, 3.95097, 4.0947, 4.27468, 4.61521, 4.83295, 4.98952, 5.33476, 5.45049, 5.53689, 5.65404, 5.68954, 5.69577, 6, 6, 6, 6, 6, 6, 6, 6, 6, 6, 6, 6, 6, 6 |
| 0 | -3 | 0.909444, 1.24682, 1.81268, 1.87515, 2.26785, 2.42692, 2.45226, 2.68236, 2.68873, 2.69623, 2.71097, 2.83751, 2.86866, 3.0833, 3.17442, 3.46255, 3.53637, 3.61091, 3.62508, 3.70274, 3.70716, 3.75761, 3.81583, 3.87045, 3.91224 |
| 0 | -1 | 0, 0, 0, 0, 0, 0.413802, 0.908981, 1.05389, 1.30081, 1.38541, 1.3955, 1.54809, 1.58387, 1.65287, 1.79789, 2.02685, 2.03425, 2.1074, 2.14812, 2.18883, 2.25233, 2.26725, 2.34345, 2.34722, 2.39965 |

| | | |
|---|---|---|
| 0 | 1 | 0, 0, 0, 0, 0, 0.25257, 0.617268, 0.732368, 1.06066, 1.19296, 1.33466, 1.36486, 1.50094, 1.50419, 1.57575, 1.8272, 1.87861, 1.97378, 2.047, 2.07648, 2.1273, 2.29686, 2.32901, 2.34636, 2.3514 |
| 0 | 3 | 0.619948, 0.978238, 1.62509, 1.78032, 2, 2.07209, 2.10224, 2.14532, 2.64204, 2.97321, 3.08415, 3.09328, 3.10497, 3.14044, 3.15505, 3.27437, 3.28227, 3.30075, 3.30514, 3.31308, 3.32364, 3.44001, 3.47591, 3.57144, 3.58261 |
| 0 | 5 | 2, 2.377, 3.11616, 3.18847, 3.65923, 3.7773, 4, 4, 4, 4, 4.46766, 4.65156, 4.72022, 4.75176, 5.12373, 5.12373, 5.12373, 5.15255, 5.17348, 5.31212, 5.49156, 5.58102, 5.62539, 5.80394, 5.80394 |
| 0 | 7 | 4, 4.38197, 5.13919, 6.61803, 6.7459, 9.11491 |
| 1 | -7 | 6 |
| 1 | -5 | 3.95097, 4.61521, 5.69577, 6, 6, 6, 6, 6, 6, 6.20166, 6.84308, 8, 8, 8, 8, 8, 8, 8, 8, 8, 8, 8, 8.27283, 8.38457, 8.85535 |
| 1 | -3 | 2.42692, 2.68873, 2.71097, 3.61091, 3.70274, 3.70716, 3.89116, 4.05108, 4.06327, 4.11613, 4.2325, 4.57143, 4.6437, 4.66931, 4.72531, 4.84061, 4.89758, 5.16831, 5.22893, 5.35233, 5.43884, 5.49621, 5.61238, 5.63402, 5.64375 |

| | | |
|---|---|---|
| 1 | -1 | 0.908981, 1.05389, 1.58387, 1.65287, 2.1074, 2.18883, 2.26377, 2.26725, 2.42892, 2.61638, 2.77559, 2.82649, 2.94656, 2.95028, 3.08255, 3.12492, 3.30109, 3.37352, 3.4606, 3.52583, 3.53822, 3.60015, 3.67623, 3.68101, 3.73982 |
| 1 | 1 | 0, 0, 0, 0.25257, 0.732368, 0.809669, 1.06066, 1.36486, 1.50094, 1.57575, 1.60454, 1.8272, 1.87861, 1.95812, 1.97378, 2.047, 2.15635, 2.29686, 2.32901, 2.34636, 2.40684, 2.41067, 2.48152, 2.52501, 2.5268 |
| 1 | 3 | 0, 0, 0, 0, 0.619948, 0.650466, 0.978238, 1.18694, 1.26674, 1.62509, 1.65547, 1.69933, 1.78032, 1.84314, 1.90844, 2.01549, 2.07209, 2.10224, 2.14532, 2.58236, 2.60342, 2.64204, 2.74067, 2.80151, 2.85624 |
| 1 | 5 | 0.62421, 1.83797, 2, 2.12091, 2.18868, 2.30431, 2.377, 2.50382, 2.64817, 3.06611, 3.11616, 3.12963, 3.18847, 3.21235, 3.2539, 3.41222, 3.43897, 3.58129, 3.62229, 3.65923, 3.72895, 3.7773, 3.87786, 3.93029, 4 |
| 1 | 7 | 2, 3.26795, 4, 4, 4, 4, 4.30766, 4.38197, 4.38197, 4.38197, 4.41819, 4.77724, 5.13919, 5.13919, 5.13919, 5.20112, 5.37357, 6.61803, 6.61803, 6.61803, 6.73205, 6.73566, 6.7459, 6.7459, 6.7459 |

| | | |
|---|---|---|
| 1 | 9 | 4 |
| 2 | -5 | 6, 8, 8, 10 |
| 2 | -3 | 3.89116, 4.57143, 5.64375, 5.67122, 5.98262, 6.23928, 6.62284, 6.6811, 7.01501, 7.55752, 7.58268, 7.58364, 7.87969, 8, 8, 8, 8, 8, 8, 8, 8, 8, 8, 8, 8 |
| 2 | -1 | 2.26377, 2.61638, 3.68101, 3.78827, 4.05304, 4.20186, 4.40859, 4.51751, 4.55636, 4.66083, 4.70743, 4.89963, 5.08492, 5.13511, 5.24163, 5.28973, 5.32069, 5.4374, 5.53123, 5.60997, 5.65758, 5.6814, 5.73473, 5.73637, 5.81463 |
| 2 | 1 | 0.809669, 1.60454, 1.95812, 2.15635, 2.40684, 2.5268, 2.6195, 2.75032, 2.77905, 2.8603, 2.87731, 2.91592, 2.91792, 3.05795, 3.29482, 3.31357, 3.40949, 3.50705, 3.57033, 3.6069, 3.72235, 3.86085, 4.01772, 4.03233, 4.04656 |
| 2 | 3 | 0, 0, 0, 0.650466, 0.981874, 1.18694, 1.26674, 1.65547, 1.69933, 1.84314, 1.84669, 1.90844, 2.01549, 2.20605, 2.58236, 2.60342, 2.73973, 2.74067, 2.80151, 2.85624, 2.87974, 2.97226, 2.97839, 3.07512, 3.14432 |

| | | |
|---|---|---|
| 2 | 5 | 0, 0, 0, 0.587208, 0.62421, 1.39209, 1.66812, 1.83797, 1.91265, 2.12091, 2.18868, 2.30431, 2.32644, 2.34828, 2.46435, 2.50382, 2.64817, 2.72374, 2.80362, 2.82684, 2.98892, 3.06611, 3.12963, 3.14667, 3.21235 |
| 2 | 7 | 1.96036, 2, 2.21873, 3.1107, 3.26795, 3.49231, 4, 4, 4, 4, 4, 4, 4.30766, 4.31402, 4.38197, 4.38197, 4.38197, 4.40411, 4.41819, 4.42139, 4.57296, 4.59457, 4.77724, 4.84232, 5.13919 |
| 2 | 9 | 4, 4, 4, 4 |
| 3 | -3 | 8, 8, 8, 12, 12, 12 |
| 3 | -1 | 5.32069, 5.93009, 5.9455, 6.14211, 6.62323, 6.65678, 7.00047, 7.77467, 7.81072, 7.99151, 8.07393, 8.32186, 8.59041, 8.83505, 9.21749, 9.41052, 9.72619, 10, 10, 10, 10, 10, 10, 10, 10 |
| 3 | 1 | 2.87731, 3.31357, 4.04656, 4.40288, 4.4323, 4.63801, 4.7851, 4.84858, 5.05349, 5.31076, 5.33925, 5.3904, 5.40525, 5.42311, 5.5334, 5.53441, 5.6165, 5.64014, 5.68437, 5.687, 5.77812, 5.80142, 5.82884, 5.87941, 5.87995 |

| | | |
|---|---|---|
| 3 | 3 | 0.981874, 1.84669, 2.20605, 2.685, 2.73973, 2.91064, 3.07512, 3.14432, 3.14703, 3.20316, 3.28305, 3.29602, 3.4404, 3.61524, 3.71777, 3.74193, 3.74312, 3.82101, 3.84254, 4.21417, 4.28024, 4.31436, 4.40656, 4.44597, 4.59753 |
| 3 | 5 | 0, 0.587208, 0.974564, 1.32907, 1.39209, 1.66812, 1.91265, 2.19701, 2.32644, 2.34828, 2.46435, 2.55201, 2.72374, 2.80362, 2.82684, 2.98892, 3.14667, 3.17156, 3.24882, 3.49624, 3.62798, 3.67153, 3.6784, 3.69554, 3.80998 |
| 3 | 7 | 0, 0, 0, 0.652205, 1.96036, 2.11219, 2.21873, 2.39713, 2.54233, 2.9358, 3.1107, 3.21776, 3.31564, 3.49231, 4, 4, 4, 4.12671, 4.19786, 4.31402, 4.38197, 4.40411, 4.42139, 4.56992, 4.56992 |
| 3 | 9 | 4, 4, 4, 4, 4, 4 |
| 4 | -1 | 10, 10, 10, 10, 10, 10, 10, 14, 14, 14 |
| 4 | 1 | 5.31076, 5.3904, 5.5334, 5.59118, 5.64014, 5.82884, 8.11388, 8.27658, 8.38197, 8.66729, 8.83089, 9.3353, 9.38919, 9.38919, 9.38919, 9.47523, 9.62093, 9.6513, 9.81139, 10.0113, 10.3461, 10.5381, 10.5638, 10.618, 10.8061 |

| | | |
|---|---|---|
| 4 | 3 | 2.685, 2.91064, 3.28305, 3.53997, 3.82101, 4.15247, 4.31436, 4.80785, 5.04673, 5.19204, 5.59647, 5.85258, 5.92084, 5.94462, 6.10848, 6.34897, 6.3899, 6.53094, 6.56511, 6.69397, 6.9042, 6.97165, 7.14762, 7.29838, 7.29838 |
| 4 | 5 | 0.974564, 1.32907, 2.16197, 2.19701, 2.37135, 2.55201, 3.17156, 3.49624, 3.5363, 3.67153, 3.80998, 4.07064, 4.12209, 4.15152, 4.28521, 4.40995, 4.53523, 4.65036, 5.0416, 5.09783, 5.167, 5.20616, 5.45671, 5.6414, 5.69068 |
| 4 | 7 | 0, 0.652205, 1.06617, 1.28037, 2.11219, 2.26441, 2.39713, 2.54233, 2.81285, 2.9358, 3.21776, 3.31564, 3.43302, 3.95431, 4.12671, 4.19786, 4.38237, 4.56992, 4.56992, 4.56992, 4.77451, 5.11811, 5.35251, 5.38197, 5.38197 |
| 4 | 9 | 0, 0.295293, 0.651313, 2.35474, 2.96274, 3.96725, 4, 4, 4, 9.76867 |
| 5 | -1 | 10 |
| 5 | 1 | 5.59118, 8.38197, 9.6513, 10.618, 11.3189, 14.4386 |
| 5 | 3 | 3.53997, 4.15247, 5.92084, 6.3899, 6.9042, 7.54625, 8.32671, 9.32942, 9.75234, 10.5178, 11.6404, 12.3854, 13.3334, 14.3946, 15.8662 |

| | | |
|---|---|---|
| 5 | 5 | 2.16197, 2.37135, 3.5363, 4.12209, 4.28521, 5.167, 5.45671, 6.10074, 6.83359, 7.08884, 7.32232, 7.83708, 9.03047, 10.2559, 10.9192, 11.9831, 12.5601, 13.2162, 13.982, 15.7698 |
| 5 | 7 | 1.06617, 1.28037, 2.26441, 2.81285, 3.43302, 3.95431, 4.38237, 5.11811, 5.53335, 6.45074, 7.06134, 10.1029, 10.8282, 12.019, 13.6929 |
| 5 | 9 | 0.295293, 0.651313, 2.35474, 2.96274, 3.96725, 9.76867 |
| 5 | 11 | 0 |

Table 17: Khovanov Laplacian nonempty spectra for $L = 10_7 1$. The planar diagram used is PD[X[1, 4, 2, 5], X[3, 8, 4, 9], X[11, 15, 12, 14], X[5, 13, 6, 12], X[13, 7, 14, 6], X[9, 19, 10, 18], X[15, 20, 16, 1], X[19, 16, 20, 17], X[17, 11, 18, 10], X[7, 2, 8, 3]].

| Homological Grading $r$ | Quantum Grading $q$ | Spectra $S_L^{r,q}$ |
|---|---|---|
| -5 | -11 | 0 |
| -5 | -9 | 0.750309, 1.39558, 1.59489, 3.4772, 5.13308, 7.64894 |
| -5 | -7 | 2.02171, 2.27124, 2.56208, 2.81422, 4.06418, 4.55491, 5.30338, 5.61645, 6.51369, 7.09077, 7.91681, 8.39056, 8.87312, 9.17769, 12.8292 |
| -5 | -5 | 3.46315, 3.58902, 3.6946, 5.03024, 5.23727, 5.85953, 6.16502, 6.9162, 7.23696, 7.75576, 8.06868, 8.42913, 8.87339, 9.26095, 9.53171, 10.3522, 10.9861, 11.5816, 13.142, 14.8265 |
| -5 | -3 | 4.70273, 6.00872, 6.21325, 7.04831, 7.25383, 7.85627, 8.67232, 9.46354, 9.78056, 10.1808, 10.859, 11.3967, 12.5498, 12.7061, 15.308 |

| | | |
|---|---|---|
| -5 | -1 | 7, 8.30573, 9.1783, 10.3942, 11.5163, 13.6055 |
| -5 | 1 | 10 |
| -4 | -9 | 0, 0, 0.750309, 1.39558, 1.59489, 2, 2, 3.4772, 5.13308, 7.64894 |
| -4 | -7 | 0, 0.815644, 1.29613, 1.49024, 1.64961, 1.94323, 2.02171, 2.27124, 2.48865, 2.56208, 2.81422, 2.83969, 3.1911, 3.30884, 3.32656, 3.51949, 3.63202, 3.96487, 4.06418, 4.16271, 4.2589, 4.49366, 4.55491, 4.83208, 4.8471 |
| -4 | -5 | 1.29862, 1.77781, 1.86556, 2.47873, 2.82568, 3.2168, 3.22278, 3.46315, 3.49705, 3.58902, 3.6946, 3.82618, 3.94999, 3.99509, 4.31861, 4.68195, 4.69407, 4.69689, 4.76506, 4.94077, 5.03024, 5.0853, 5.23727, 5.25839, 5.36153 |
| -4 | -3 | 2.83569, 3.30589, 4.01008, 4.48007, 4.5494, 4.70273, 4.88294, 5.21714, 5.33301, 5.55393, 5.75742, 5.84667, 6.00872, 6.01029, 6.18273, 6.21325, 6.32804, 6.4226, 6.59896, 6.71647, 6.9943, 7.04831, 7.05538, 7.16527, 7.25383 |
| -4 | -1 | 5.61958, 5.90257, 6.65319, 6.66711, 6.87272, 7, 7.29779, 7.5347, 8.00776, 8.13226, 8.30494, 8.30573, 8.34456, 8.66298, 9.0889, 9.14433, 9.1783, 9.22415, 9.28151, 9.36212, 9.78924, 9.83666, 9.84188, 10.1867, 10.2589 |

| | | |
|---|---|---|
| -4 | 1 | 10, 10, 10, 10, 10, 10, 10, 10, 12, 12 |
| -3 | -9 | 2, 2 |
| -3 | -7 | 0, 0, 0, 0, 0.815644, 1.29613, 1.49024, 1.64961, 1.94323, 2, 2, 2, 2.48865, 2.62164, 2.83969, 3, 3.08503, 3.18481, 3.1911, 3.30884, 3.32656, 3.49364, 3.51949, 3.63202, 3.96487 |
| -3 | -5 | 0, 0, 0.580323, 0.899931, 1.20034, 1.29862, 1.41546, 1.49625, 1.60297, 1.76301, 1.77781, 1.86556, 1.98661, 2.25711, 2.47873, 2.79961, 2.82568, 2.908, 3.01383, 3.2168, 3.22278, 3.29971, 3.49328, 3.49705, 3.62653 |
| -3 | -3 | 1.49011, 1.67166, 1.76278, 1.90959, 2.33522, 2.41743, 2.44888, 2.55599, 2.83569, 3.00365, 3.04594, 3.09674, 3.11761, 3.30589, 3.44128, 3.47121, 3.57691, 3.88864, 3.90043, 4.01008, 4.29964, 4.34172, 4.38199, 4.48007, 4.53193 |
| -3 | -1 | 2.99122, 3.65419, 3.76617, 4.10237, 4.47668, 4.57223, 4.8518, 4.86281, 5.22993, 5.24156, 5.25242, 5.40719, 5.58103, 5.61958, 5.62141, 5.70824, 5.81743, 5.90257, 6.07162, 6.08571, 6.30092, 6.44065, 6.52979, 6.54261, 6.65319 |

| | | |
|---|---|---|
| -3 | 1 | 5.4037, 5.4387, 5.81719, 6.83707, 7.21598, 7.53046, 8.3228, 8.37633, 9.6564, 10, 10, 10, 10, 10, 10, 10, 10, 10, 10, 10, 10, 10, 10, 10, 10 |
| -3 | 3 | 8, 8 |
| -2 | -7 | 2, 2, 2, 2.62164, 3, 3.08503, 3.18481, 3.49364, 4, 4, 4, 4, 4, 4.25791, 4.64006, 5.21072, 6.57464, 9.361, 9.57054 |
| -2 | -5 | 0, 0, 0, 0, 0, 0, 0.580323, 0.899931, 1.20034, 1.41546, 1.49625, 1.60297, 1.76301, 1.8121, 1.8358, 1.98661, 2, 2.21973, 2.25711, 2.79961, 2.908, 3, 3.01383, 3.02683, 3.07127 |
| -2 | -3 | 0, 0, 0, 0, 0.893236, 0.969055, 1.05805, 1.07837, 1.22931, 1.49011, 1.63862, 1.66199, 1.67166, 1.69316, 1.76278, 1.90959, 1.94959, 1.9934, 2.25539, 2.30082, 2.33522, 2.37055, 2.37626, 2.40518, 2.41743 |
| -2 | -1 | 1.49523, 1.62111, 1.8124, 1.87691, 1.92249, 1.92543, 2.3859, 2.39873, 2.46052, 2.48108, 2.90336, 2.99122, 3.02697, 3.13682, 3.21452, 3.30563, 3.50296, 3.60681, 3.61549, 3.65419, 3.67869, 3.69506, 3.76462, 3.76617, 3.89055 |

| | | |
|---|---|---|
| -2 | 1 | 3.53511, 3.57963, 3.8729, 4.3281, 4.34946, 4.60743, 4.68747, 4.76115, 4.8523, 4.9394, 5.33774, 5.378, 5.37961, 5.4037, 5.4387, 5.51549, 5.59294, 5.69635, 5.81719, 5.98299, 6.12497, 6.28069, 6.49565, 6.49591, 6.50382 |
| -2 | 3 | 7, 7, 7.43845, 8, 8, 8, 8, 8, 8, 8, 8, 8, 8, 8, 8, 8, 10, 10, 11.5616 |
| -1 | -7 | 4, 4 |
| -1 | -5 | 1.8121, 1.8358, 2, 2.21973, 3, 3.02683, 3.07127, 3.19752, 3.48307, 4, 4, 4, 4.21989, 4.23127, 4.31527, 4.32438, 4.45578, 4.55753, 4.56152, 4.60983, 4.78982, 4.78982, 4.82413, 4.87452, 4.93953 |
| -1 | -3 | 0, 0, 0, 0, 0, 0, 0.893236, 0.969055, 1.05805, 1.07837, 1.22931, 1.63862, 1.63879, 1.64657, 1.66199, 1.69316, 1.76334, 1.86147, 1.94959, 1.97786, 1.9934, 2.05168, 2.14839, 2.25539, 2.30082 |
| -1 | -1 | 0, 0, 0, 0, 0, 0, 0.44328, 0.818838, 1.16457, 1.328, 1.34402, 1.43741, 1.49523, 1.50556, 1.62111, 1.8124, 1.87691, 1.92249, 1.92543, 1.93564, 1.99008, 2.01724, 2.12266, 2.13699, 2.23779 |

| | | |
|---|---|---|
| -1 | 1 | 1.45903, 1.79781, 1.82133, 1.88505, 1.91562, 1.93535, 1.93894, 2.31617, 2.51887, 2.92419, 3.11099, 3.18688, 3.21825, 3.35572, 3.53232, 3.53511, 3.57963, 3.60607, 3.63416, 3.78926, 3.79379, 3.8371, 3.84328, 3.8729, 3.92885 |
| -1 | 3 | 3.20388, 3.30046, 4.59032, 5.1775, 5.53382, 5.90697, 6, 6.5359, 6.5359, 7, 7, 7, 7, 7, 7, 7, 7, 7.0007, 7.1206, 7.17157, 7.23219, 7.35425, 7.35425, 7.38053, 7.43845 |
| -1 | 5 | 6, 6 |
| 0 | -5 | 4, 4.55753, 4.78982, 5, 5, 5.38977, 6, 6, 6, 6, 6, 6, 6, 6, 6, 6, 6.73929, 6.87818, 10.4709, 11.1745 |
| 0 | -3 | 1.63879, 1.64657, 1.76334, 1.86147, 1.97786, 2.05168, 2.14839, 2.59266, 2.82355, 3.14942, 3.20987, 3.29945, 3.44664, 3.59516, 3.64048, 3.69587, 3.70774, 3.73765, 3.87751, 3.96398, 4.00163, 4.06279, 4.06472, 4.12082, 4.16599 |
| 0 | -1 | 0, 0, 0, 0, 0, 0, 0, 0.44328, 0.818838, 1.16457, 1.328, 1.34402, 1.43741, 1.50556, 1.8201, 1.93099, 1.93356, 1.93564, 1.95198, 1.99008, 1.9978, 2.01724, 2.08327, 2.12266, 2.13699 |

| | | |
|---|---|---|
| 0 | 1 | 0, 0, 0, 0, 0, 0, 0, 0.494418, 0.751065, 0.936282, 1.40784, 1.42978, 1.43896, 1.45903, 1.46074, 1.69436, 1.77169, 1.79781, 1.82133, 1.88505, 1.91562, 1.93535, 1.93894, 1.99054, 2.05596 |
| 0 | 3 | 1.52102, 1.63964, 1.64657, 1.86204, 1.93682, 2.4246, 2.46267, 2.56451, 2.57062, 2.89266, 3.07114, 3.20388, 3.29749, 3.30046, 3.42146, 3.47134, 3.5988, 3.70774, 3.86289, 4.00987, 4.1516, 4.27222, 4.31795, 4.41089, 4.59032 |
| 0 | 5 | 4, 5, 5, 5, 5.17157, 5.43845, 6, 6, 6, 6, 6, 6, 6, 6, 6, 6, 6, 6, 6, 6, 6, 6, 6, 8, 9.56155, 10.8284 |
| 1 | -5 | 6, 6 |
| 1 | -3 | 3.69587, 3.73765, 4.12082, 4.80011, 5.11243, 5.39445, 6, 6.1459, 6.62772, 6.70742, 7, 7, 7, 7, 7, 7, 7, 7.12677, 7.16756, 7.1919, 7.29844, 7.29844, 7.35425, 7.42165, 7.43845 |
| 1 | -1 | 1.8201, 1.93099, 1.93356, 1.95198, 1.9978, 2.08327, 2.26245, 2.27945, 2.54883, 2.92418, 3.00771, 3.15458, 3.17893, 3.26711, 3.3076, 3.35067, 3.49572, 3.55003, 3.565, 3.64666, 3.68325, 3.79638, 3.82526, 3.85137, 4.001 |

| | | |
|---|---|---|
| 1 | 1 | 0, 0, 0, 0, 0, 0, 0.494418, 0.751065, 0.936282, 1.16906, 1.40784, 1.42978, 1.43896, 1.46074, 1.50321, 1.69436, 1.77169, 1.79105, 1.96546, 1.99054, 2.05596, 2.14443, 2.1849, 2.25353, 2.35877 |
| 1 | 3 | 0, 0, 0, 0, 0, 0, 0.489772, 0.979261, 1.26087, 1.26101, 1.32929, 1.48191, 1.51776, 1.52102, 1.63964, 1.64657, 1.70757, 1.73816, 1.81546, 1.86204, 1.93682, 2.00792, 2.32875, 2.4246, 2.46267 |
| 1 | 5 | 1.47912, 1.96562, 2, 2, 2.62413, 2.62853, 3.46758, 3.55664, 3.58579, 3.59361, 4, 4, 4.2507, 4.39445, 4.63986, 4.66411, 4.74123, 4.84584, 5, 5, 5, 5, 5, 5, 5 |
| 1 | 7 | 4, 4 |
| 2 | -3 | 7, 7, 7.43845, 8, 8, 8, 8, 8, 8, 8, 8, 8, 8, 8, 8, 8, 8, 11.5616, 12 |
| 2 | -1 | 3.49572, 3.55003, 3.64666, 4.17879, 4.63499, 4.72679, 4.91177, 4.92057, 5.1787, 5.25415, 5.36231, 5.40464, 5.42333, 5.47807, 5.47982, 5.60288, 5.73708, 5.80308, 5.85748, 5.93255, 5.95169, 6.17135, 6.22272, 6.30002, 6.41097 |

| | | |
|---|---|---|
| 2 | 1 | 1.16906, 1.50321, 1.79105, 1.96546, 2.1849, 2.36343, 2.57889, 2.59044, 2.82055, 2.84542, 2.88541, 2.99467, 3.03251, 3.05452, 3.08375, 3.18002, 3.33952, 3.37207, 3.64662, 3.68728, 3.74101, 3.83349, 3.86265, 3.8664, 3.97925 |
| 2 | 3 | 0, 0, 0, 0, 0.489772, 0.979261, 1.24962, 1.26087, 1.26101, 1.32929, 1.48191, 1.51776, 1.56067, 1.63215, 1.6399, 1.70757, 1.73816, 1.81546, 1.82915, 2.00792, 2.32875, 2.52058, 2.55541, 2.62204, 2.67497 |
| 2 | 5 | 0, 0, 0, 0, 0, 0, 0.379121, 0.612724, 1.4743, 1.47912, 1.6249, 1.73811, 1.85273, 1.96562, 2, 2, 2.01074, 2.08432, 2.62413, 2.62853, 2.65621, 3.02963, 3.03282, 3.27098, 3.29207 |
| 2 | 7 | 2, 2, 2, 2.41356, 2.64127, 3, 3.48486, 4, 4, 4, 4, 4, 4, 4.3425, 4.76511, 5.58161, 5.70347, 9.43462, 9.63299 |
| 3 | -3 | 8, 8 |
| 3 | -1 | 4.92057, 5.40464, 6.55654, 6.73188, 7.55051, 7.63724, 7.63793, 8.21058, 9.4823, 9.5114, 10, 10, 10, 10, 10, 10, 10, 10, 10, 10, 10, 10, 10, 10, 10 |

| | | |
|---|---|---|
| 3 | 1 | 2.84542, 3.18002, 3.64662, 3.83349, 4.28688, 5.05936, 5.19665, 5.22278, 5.27199, 5.28828, 5.31134, 5.40404, 5.57002, 5.73111, 5.80379, 5.93279, 6.00767, 6.01873, 6.04182, 6.05477, 6.19257, 6.31541, 6.38756, 6.41572, 6.46084 |
| 3 | 3 | 1.24962, 1.56067, 1.63215, 1.6399, 1.82915, 2.78761, 2.91865, 3.00229, 3.01654, 3.16617, 3.20731, 3.4053, 3.41035, 3.5192, 3.53177, 3.79725, 3.84429, 3.93746, 3.99522, 4.00608, 4.13872, 4.21893, 4.32619, 4.42182, 4.43541 |
| 3 | 5 | 0, 0, 0.379121, 0.612724, 1.25437, 1.4743, 1.58047, 1.6249, 1.73811, 1.85273, 2.01074, 2.08432, 2.34682, 2.47171, 2.63121, 2.65621, 2.98541, 3.02963, 3.03282, 3.26004, 3.27098, 3.29207, 3.46771, 3.53387, 3.60787 |
| 3 | 7 | 0, 0, 0, 0, 0.738892, 0.952758, 1.94526, 2, 2, 2, 2.27543, 2.30974, 2.41356, 2.59368, 2.64127, 2.65101, 2.82734, 3, 3.2996, 3.32121, 3.48486, 3.53327, 3.55867, 3.85441, 4 |
| 3 | 9 | 2, 2 |
| 4 | -1 | 10, 10, 10, 10, 10, 10, 10, 10, 12, 12 |

| | | |
|---|---|---|
| 4 | 1 | 5.28828, 6.04182, 6.46084, 6.55686, 6.78356, 6.90649, 6.95489, 7.79837, 7.89892, 8.15685, 8.29253, 8.35198, 8.35264, 8.56231, 8.73799, 9.14008, 9.28814, 9.80383, 9.8839, 9.90441, 10, 10.0547, 10.2169, 10.277, 10.4808 |
| 4 | 3 | 3.01654, 3.4053, 3.79725, 4.00608, 4.53422, 4.819, 4.88867, 4.97437, 5.23635, 5.32153, 5.47908, 5.6503, 5.80175, 5.88284, 6.01566, 6.14688, 6.29017, 6.49866, 6.56676, 6.61589, 6.73546, 6.95125, 7.00726, 7.03821, 7.09248 |
| 4 | 5 | 1.25437, 1.58047, 2.34682, 2.47171, 2.63121, 2.98541, 3.12619, 3.26004, 3.55664, 3.60787, 4.00632, 4.06629, 4.07122, 4.26846, 4.29959, 4.30305, 4.60635, 4.71138, 4.79035, 4.82226, 4.93699, 4.96723, 5.04027, 5.1555, 5.43322 |
| 4 | 7 | 0, 0.738892, 0.952758, 1.82988, 1.94526, 2.02085, 2.27543, 2.30974, 2.59368, 2.65101, 2.81527, 2.82734, 3.06818, 3.2996, 3.32121, 3.53327, 3.55867, 3.85441, 4, 4.12527, 4.26516, 4.51065, 4.51213, 4.74056, 4.85062 |
| 4 | 9 | 0, 0, 0.705698, 1, 2, 2, 2.31285, 3.37542, 4.26547, 8.34057 |
| 5 | -1 | 10 |
| 5 | 1 | 6.90649, 8.15685, 9.8839, 10.5243, 10.7657, 13.7628 |

| | | |
|---|---|---|
| 5 | 3 | 4.88867, 5.23635, 6.56676, 7.03821, 7.66181, 7.71751, 8.72076, 9.21088, 9.8062, 10.1601, 11.0059, 11.758, 12.1105, 13.0313, 15.087 |
| 5 | 5 | 3.12619, 3.55664, 4.26846, 4.82226, 5.04027, 5.91385, 6.26781, 6.6214, 7.03133, 7.56254, 7.72398, 8.17774, 9.19812, 9.68163, 10.0833, 10.295, 11.1903, 12.2753, 12.4448, 14.7191 |
| 5 | 7 | 1.82988, 2.02085, 2.81527, 3.06818, 4.12527, 4.85062, 5.0324, 5.42193, 5.74844, 6.17999, 8.23108, 8.81869, 9.1175, 10.0429, 12.697 |
| 5 | 9 | 0.705698, 1, 2.31285, 3.37542, 4.26547, 8.34057 |
| 5 | 11 | 0 |

Table 18: Khovanov Laplacian nonempty spectra for $L = 10_91$. The planar diagram used is PD[X[6, 2, 7, 1], X[20, 6, 1, 5], X[16, 9, 17, 10], X[10, 3, 11, 4], X[2, 18, 3, 17], X[14, 7, 15, 8], X[8, 15, 9, 16], X[12, 20, 13, 19], X[18, 12, 19, 11], X[4, 13, 5, 14]].

| Homological Grading $r$ | Quantum Grading $q$ | Spectra $S_L^{r,q}$ |
|---|---|---|
| -5 | -11 | 0 |
| -5 | -9 | 0.627071, 1.50743, 2.34649, 3.48204, 3.86679, 8.17017 |
| -5 | -7 | 2.00308, 2.51214, 2.86195, 3.7377, 3.80771, 4.00409, 5.1494, 5.5088, 5.93759, 6.34311, 7.26669, 8.25098, 9.89055, 10.4454, 12.2808 |

| | | |
|---|---|---|
| -5 | -5 | 3.66997, 3.87386, 4.48057, 4.87396, 5.221, 5.66409, 6.05026, 6.4074, 7.01244, 7.14349, 7.65036, 8.3259, 8.77495, 9.13054, 9.63184, 11.0732, 11.5305, 12.2227, 12.4266, 14.8365 |
| -5 | -3 | 5.40066, 5.94702, 6.17244, 6.81892, 7.50443, 7.8898, 8.3337, 8.95372, 9.30365, 10.5807, 10.6245, 11.0479, 12.9516, 13.1875, 15.2835 |
| -5 | -1 | 7.46529, 8.38197, 8.50423, 10.618, 11.1578, 13.8726 |
| -5 | 1 | 10 |
| -4 | -9 | 0, 0, 0.627071, 1.50743, 2, 2, 2.34649, 3.48204, 3.86679, 8.17017 |
| -4 | -7 | 0, 0.695635, 1.15222, 1.23707, 2.00308, 2.14743, 2.51214, 2.54458, 2.60719, 2.63763, 2.67869, 2.86195, 2.9478, 3.21835, 3.70955, 3.7112, 3.7377, 3.80771, 3.98793, 4.00409, 4.07665, 4.3442, 4.55278, 4.87478, 4.89918 |
| -4 | -5 | 0.862704, 1.94802, 2.34472, 2.8396, 2.98337, 3.08555, 3.17422, 3.64612, 3.66997, 3.69991, 3.84654, 3.87386, 3.91669, 4.00633, 4.03667, 4.0717, 4.15907, 4.48057, 4.54509, 4.56723, 4.84083, 4.87396, 4.97145, 5.03899, 5.16403 |

| | | |
|---|---|---|
| -4 | -3 | 2.48703, 3.35247, 4.10069, 4.50032, 4.80268, 4.83535, 5.14806, 5.17826, 5.40066, 5.43663, 5.50734, 5.5543, 5.68006, 5.75525, 5.82602, 5.89931, 5.94702, 6.1349, 6.17244, 6.20031, 6.34057, 6.47045, 6.55025, 6.80579, 6.81892 |
| -4 | -1 | 4.8359, 5.73775, 6.89385, 6.94798, 7.18949, 7.19299, 7.26951, 7.46529, 7.65246, 7.70746, 7.82675, 8.03294, 8.13431, 8.38197, 8.48103, 8.50423, 8.70836, 8.9601, 9.46766, 9.48742, 9.83228, 10.3278, 10.3848, 10.3948, 10.4235 |
| -4 | 1 | 10, 10, 10, 10, 10, 10, 10, 10, 12, 12 |
| -3 | -9 | 2, 2 |
| -3 | -7 | 0, 0, 0, 0, 0.695635, 1.15222, 1.23707, 2, 2.14743, 2.39804, 2.48378, 2.54458, 2.60719, 2.63763, 2.63771, 2.67869, 2.9478, 3.21835, 3.33435, 3.70955, 3.7112, 3.98793, 4, 4, 4.07665 |
| -3 | -5 | 0, 0, 0.328728, 0.455885, 0.691258, 0.862704, 1.09608, 1.94027, 1.94802, 2.19624, 2.1986, 2.3266, 2.34472, 2.46611, 2.8396, 2.98024, 2.98337, 2.9963, 2.99958, 3.08555, 3.17422, 3.27598, 3.36035, 3.46404, 3.58899 |

| | | |
|---|---|---|
| -3 | -3 | 0.998189, 1.10949, 1.35224, 1.71254, 1.77119, 1.9183, 2.31581, 2.48703, 2.74981, 2.7617, 3.01237, 3.11513, 3.28354, 3.29061, 3.35247, 3.6382, 3.75589, 3.81514, 3.88555, 4.07264, 4.10069, 4.15123, 4.3083, 4.43531, 4.50032 |
| -3 | -1 | 2.50383, 2.85491, 2.88105, 3.03189, 3.76288, 4.53396, 4.62532, 4.65752, 4.76051, 4.8359, 4.88817, 5.00827, 5.1985, 5.44953, 5.49965, 5.53515, 5.66913, 5.7344, 5.73775, 5.92195, 6.1934, 6.47465, 6.62183, 6.6542, 6.73048 |
| -3 | 1 | 4.39877, 4.87169, 6.12397, 6.1255, 7.59656, 7.90325, 8.64235, 8.77245, 9.4913, 9.51793, 10, 10, 10, 10, 10, 10, 10, 10, 10, 10, 10, 10, 10, 10, 10 |
| -3 | 3 | 8, 8 |
| -2 | -7 | 2, 2.39804, 2.48378, 2.63771, 3.33435, 4, 4, 4, 4.6802, 5, 5, 5, 5, 5, 5, 5, 5, 5.13227, 5.4424, 5.72216, 10.0593, 10.1098 |
| -2 | -5 | 0, 0, 0, 0, 0, 0.328728, 0.455885, 0.691258, 1.09608, 1.73509, 1.86172, 1.94027, 2, 2, 2.10129, 2.19624, 2.1986, 2.3266, 2.46611, 2.98024, 2.9963, 2.99958, 3.01491, 3.04172, 3.27598 |

| | | |
|---|---|---|
| -2 | -3 | 0, 0, 0, 0, 0.326251, 0.462794, 0.992665, 0.998189, 1.10949, 1.35224, 1.64505, 1.71254, 1.76568, 1.77119, 1.9183, 1.97968, 2.06978, 2.08156, 2.24426, 2.31581, 2.34107, 2.43475, 2.60228, 2.74188, 2.74981 |
| -2 | -1 | 0.989385, 1.40231, 1.42626, 1.58519, 1.71873, 2.20632, 2.38779, 2.50383, 2.59557, 2.7489, 2.85491, 2.88105, 2.89956, 2.91655, 3.03189, 3.03547, 3.06765, 3.20097, 3.32143, 3.70146, 3.72248, 3.76088, 3.76288, 3.93788, 4.06962 |
| -2 | 1 | 2.83838, 3.35083, 3.76041, 3.91214, 4.0672, 4.14954, 4.18055, 4.39877, 4.45156, 4.59217, 4.75549, 4.75651, 4.80281, 4.87169, 5.30627, 5.70863, 5.9125, 6.12397, 6.1255, 6.17264, 6.20005, 6.20256, 6.20372, 6.34778, 6.45253 |
| -2 | 3 | 7, 7, 7.35425, 7.35425, 7.43845, 7.76393, 8, 8, 8, 8, 8, 8, 8, 8, 8, 8, 8, 11.5616, 12.2361, 12.6458, 12.6458, 13 |
| -1 | -7 | 4, 5, 5, 5, 5, 5 |
| -1 | -5 | 1.73509, 1.86172, 2, 2, 2.10129, 3.01491, 3.04172, 3.07042, 3.28164, 3.69035, 3.79146, 3.80404, 4, 4, 4, 4.28801, 4.36889, 4.39908, 4.55343, 4.6258, 4.79149, 5, 5, 5, 5 |

| | | |
|---|---|---|
| -1 | -3 | 0, 0, 0, 0, 0, 0, 0.326251, 0.462794, 0.992665, 1.51309, 1.64505, 1.75579, 1.75818, 1.76568, 1.87432, 1.97968, 2.04888, 2.06978, 2.08156, 2.24426, 2.34107, 2.41371, 2.43475, 2.60228, 2.72549 |
| -1 | -1 | 0, 0, 0, 0, 0, 0.377564, 0.989385, 1.05993, 1.14493, 1.40231, 1.41302, 1.42626, 1.46978, 1.58519, 1.71873, 1.94372, 1.98209, 1.99814, 2.08653, 2.18599, 2.20632, 2.28893, 2.37445, 2.38779, 2.50585 |
| -1 | 1 | 0.765575, 0.825256, 1.41622, 2.01839, 2.61053, 2.67452, 2.76586, 2.78536, 2.83838, 2.85399, 2.88479, 3.25402, 3.35083, 3.39373, 3.46529, 3.5702, 3.63765, 3.76041, 3.76845, 3.90797, 3.91214, 3.93015, 3.96256, 4.0672, 4.07807 |
| -1 | 3 | 2.43503, 2.62723, 3.17344, 3.89047, 3.93087, 4.42688, 4.81366, 4.89567, 5.47235, 5.53733, 6.04199, 6.09161, 6.25834, 6.37076, 6.37425, 6.76186, 6.85424, 7, 7, 7, 7, 7, 7, 7, 7.19633 |
| -1 | 5 | 5, 5.76393, 6, 7, 7, 10.2361 |
| 0 | -7 | 5 |
| 0 | -5 | 3.07042, 4, 4.28801, 4.36889, 5, 5, 5, 5, 5, 5.65584, 6, 6.76393, 7, 7, 7, 7, 7, 7, 7, 7, 7, 7, 7, 7, 7 |

| | | |
|---|---|---|
| 0 | -3 | 1.51309, 1.75579, 1.75818, 1.87432, 2.04888, 2.41371, 2.72549, 2.92213, 2.93522, 3.14907, 3.36608, 3.41903, 3.56358, 3.56887, 3.63162, 3.63892, 3.84272, 3.86471, 3.95391, 4.1174, 4.19523, 4.19742, 4.2486, 4.28109, 4.36676 |
| 0 | -1 | 0, 0, 0, 0, 0, 0, 0, 0.377564, 1.05993, 1.14493, 1.15842, 1.28337, 1.41302, 1.46978, 1.74383, 1.94372, 1.98073, 1.98209, 1.99814, 2.08653, 2.11811, 2.18599, 2.22634, 2.28893, 2.37445 |
| 0 | 1 | 0, 0, 0, 0, 0, 0, 0, 0.69048, 0.765575, 0.825256, 1.08285, 1.33858, 1.37028, 1.41622, 1.45817, 1.73806, 1.80419, 1.83964, 2.01839, 2.02835, 2.11103, 2.1136, 2.20302, 2.23874, 2.28585 |
| 0 | 3 | 0.76351, 1.24297, 2.36027, 2.43503, 2.47657, 2.62723, 2.65072, 2.6896, 2.70254, 2.73767, 2.74619, 2.94382, 3.16404, 3.17344, 3.3293, 3.46608, 3.57455, 3.64605, 3.64816, 3.87085, 3.89047, 3.93087, 3.99141, 4.04366, 4.07964 |
| 0 | 5 | 2.42706, 3, 3.99454, 4.15913, 5, 5, 5, 5, 5.21917, 5.41977, 5.76393, 5.76393, 5.76393, 5.76765, 5.82315, 5.98018, 6, 6, 6, 6, 6.11706, 6.59492, 7, 7, 7 |
| 0 | 7 | 5 |
| 1 | -5 | 5, 7, 7, 7, 7, 7, 7, 7, 7.58579, 10.4142 |

| | | |
|---|---|---|
| 1 | -3 | 2.93522, 3.36608, 4.1174, 4.19523, 4.2486, 4.41628, 4.62498, 4.6826, 5.00276, 5.18263, 5.35344, 5.35673, 5.55825, 5.63557, 5.66958, 6, 6, 6.04386, 6.17545, 6.32539, 6.54573, 6.63849, 6.68846, 6.77964, 6.83772 |
| 1 | -1 | 1.15842, 1.28337, 1.74383, 1.98073, 2.11811, 2.22634, 2.57443, 2.77341, 2.95727, 3.02196, 3.09864, 3.11127, 3.1781, 3.37275, 3.6607, 3.67861, 3.79121, 3.8061, 3.84668, 3.8539, 3.90584, 3.92574, 4.06012, 4.09477, 4.26867 |
| 1 | 1 | 0, 0, 0, 0, 0, 0.69048, 1.06814, 1.08285, 1.33858, 1.37028, 1.45817, 1.63144, 1.73806, 1.80419, 1.83964, 1.92417, 1.95606, 2.02835, 2.03578, 2.11103, 2.1136, 2.20302, 2.23874, 2.27284, 2.28585 |
| 1 | 3 | 0, 0, 0, 0, 0, 0, 0.631306, 0.76351, 0.992804, 1.15033, 1.24297, 1.27555, 1.46295, 2.01798, 2.02242, 2.17471, 2.29338, 2.36027, 2.47657, 2.59933, 2.64163, 2.65072, 2.65735, 2.6896, 2.70254 |
| 1 | 5 | 1.28543, 1.77804, 2.42706, 2.43175, 2.5511, 2.58411, 2.61522, 2.80297, 3, 3, 3, 3.37059, 3.60933, 3.80887, 3.99454, 4, 4.10636, 4.15913, 4.15913, 4.22079, 4.27141, 4.32414, 4.54813, 4.85901, 4.87679 |
| 1 | 7 | 3, 3.41266, 4.15328, 5, 5, 5, 5, 5.71933, 6.45791, 9.25682 |

| | | |
|---|---|---|
| 2 | -5 | 7 |
| 2 | -3 | 4.41628, 5.35344, 6.68846, 7, 7.36015, 7.55051, 7.55051, 8, 8, 8, 8, 8, 8, 8, 8, 8, 8, 8, 8, 8.27745, 8.55092, 9.36258, 11, 11, 11, 11 |
| 2 | -1 | 2.57443, 3.1781, 3.90584, 4.4697, 4.54937, 4.68613, 4.70667, 4.81967, 5.06907, 5.11757, 5.11903, 5.17895, 5.30404, 5.39343, 5.46273, 5.50544, 5.55784, 5.58565, 5.59352, 5.74643, 5.79911, 6.20082, 6.23622, 6.24105, 6.29957 |
| 2 | 1 | 1.06814, 1.63144, 1.92417, 1.95606, 2.03578, 2.27284, 2.46126, 2.64516, 3.09972, 3.14422, 3.17459, 3.27131, 3.5411, 3.6304, 3.66861, 3.71427, 3.72769, 3.75137, 3.76322, 3.78402, 3.79977, 3.8697, 3.88444, 3.90381, 3.94525 |
| 2 | 3 | 0, 0, 0, 0, 0.631306, 0.992804, 1.15033, 1.27555, 1.37415, 1.46295, 1.47752, 1.87698, 2.01798, 2.02242, 2.02742, 2.17471, 2.29338, 2.45405, 2.47455, 2.59933, 2.64163, 2.65735, 2.76409, 2.89503, 2.89512 |
| 2 | 5 | 0, 0, 0, 0, 0, 0.615375, 1.28543, 1.2882, 1.53817, 1.5529, 1.65761, 1.77804, 2.29547, 2.43175, 2.44759, 2.48683, 2.5511, 2.58411, 2.61522, 2.80297, 2.8336, 3, 3, 3.05208, 3.07629 |

| | | |
|---|---|---|
| 2 | 7 | 1.38153, 2.4482, 3, 3, 3, 3.41266, 3.41266, 3.44406, 3.69388, 4.15328, 4.15328, 4.18735, 4.352, 5, 5, 5, 5, 5, 5, 5.71933, 5.71933, 5.81687, 5.96528, 6.45791, 6.45791 |
| 2 | 9 | 3 |
| 3 | -3 | 8, 8, 11 |
| 3 | -1 | 5.11903, 5.50544, 6.29957, 6.4078, 7.09394, 7.93125, 7.9458, 8.19974, 8.46333, 9.33992, 9.5788, 9.96375, 10, 10, 10, 10, 10, 10, 10, 10, 10, 10, 10, 10, 10 |
| 3 | 1 | 3.17459, 3.71427, 3.8697, 3.88444, 4.38878, 4.42136, 4.69527, 4.70621, 4.74861, 4.84718, 4.9703, 5.0384, 5.43275, 5.48991, 5.70491, 5.87228, 6.02776, 6.1148, 6.18279, 6.22394, 6.26633, 6.29566, 6.38314, 6.39584, 6.45263 |
| 3 | 3 | 1.37415, 1.47752, 1.87698, 2.02742, 2.43923, 2.45405, 2.47455, 2.76409, 2.95618, 3.2185, 3.28636, 3.46926, 3.54964, 3.6443, 3.75814, 3.84899, 3.97293, 3.98, 4.21522, 4.22799, 4.26379, 4.26883, 4.40666, 4.46595, 4.4899 |
| 3 | 5 | 0, 0, 0.615375, 0.93671, 1.2882, 1.53817, 1.5529, 1.65761, 1.72105, 2.29547, 2.37175, 2.44759, 2.48683, 2.8165, 2.8336, 3.05208, 3.07629, 3.08646, 3.11004, 3.19897, 3.2836, 3.29248, 3.40006, 3.49125, 3.61097 |

| | | |
|---|---|---|
| 3 | 7 | 0, 0, 0, 0, 0.873241, 1.00506, 1.38153, 1.77431, 2.30488, 2.4482, 2.6104, 2.96956, 3, 3, 3.17876, 3.30459, 3.41266, 3.44406, 3.56261, 3.66869, 3.66869, 3.69388, 3.7557, 4.05263, 4.15328 |
| 3 | 9 | 3, 3, 3 |
| 4 | -1 | 10, 10, 10, 10, 10, 10, 10, 10, 13, 13 |
| 4 | 1 | 4.70621, 6.18279, 6.38314, 6.51516, 6.55991, 6.68648, 6.85736, 7.95558, 8.09122, 8.20972, 8.38197, 8.4089, 8.61221, 8.61221, 8.89188, 9.177, 9.33345, 9.39518, 9.56379, 9.70039, 9.86778, 10.2245, 10.3433, 10.4937, 10.5312 |
| 4 | 3 | 2.43923, 3.54964, 3.97293, 4.26883, 4.40423, 4.40666, 4.71448, 5.02214, 5.14025, 5.51636, 5.63823, 5.77467, 5.95359, 6.15343, 6.25432, 6.34624, 6.43648, 6.48342, 6.48342, 6.56419, 6.66195, 6.69879, 6.87782, 7.02503, 7.02637 |
| 4 | 5 | 0.93671, 1.72105, 2.37175, 2.62764, 2.8165, 3.08646, 3.19897, 3.49125, 3.56852, 3.87176, 3.92899, 4.05877, 4.08596, 4.24654, 4.37333, 4.47701, 4.64654, 4.66551, 4.80793, 4.95225, 4.95225, 4.98042, 5.11359, 5.17734, 5.25514 |

| | | |
|---|---|---|
| 4 | 7 | 0, 0.873241, 1.00506, 1.29815, 1.77431, 2.25032, 2.30488, 2.6104, 2.96956, 3.08937, 3.17876, 3.30459, 3.33056, 3.56261, 3.66869, 3.66869, 3.70831, 3.7557, 4.05263, 4.31159, 4.31228, 4.38197, 4.38197, 4.60519, 4.86409 |
| 4 | 9 | 0, 0, 0.426237, 1.21714, 2.62807, 3, 3, 3.22891, 3.91704, 8.5826 |
| 5 | -1 | 10 |
| 5 | 1 | 6.55991, 8.38197, 9.39518, 10.618, 11.0952, 13.9498 |
| 5 | 3 | 4.40423, 5.14025, 6.66195, 7.02503, 7.43907, 7.73746, 8.13475, 9.06498, 9.43721, 10.4989, 11.2134, 11.8846, 12.4099, 13.576, 15.3723 |
| 5 | 5 | 2.62764, 3.56852, 4.37333, 4.64654, 5.11359, 5.63106, 5.9715, 6.4064, 6.85935, 7.23384, 7.63297, 8.05419, 8.93665, 9.73497, 10.0451, 11.3007, 11.5453, 12.3712, 12.8624, 15.0848 |
| 5 | 7 | 1.29815, 2.25032, 3.08937, 3.33056, 3.70831, 4.31228, 4.86409, 5.14767, 6.16282, 6.17762, 7.16674, 9.01522, 10.0404, 10.7471, 12.6893 |
| 5 | 9 | 0.426237, 1.21714, 2.62807, 3.22891, 3.91704, 8.5826 |
| 5 | 11 | 0 |

Table 19: Khovanov Laplacian nonempty spectra for $L = 10_104$. The planar diagram used is PD[X[6, 2, 7, 1], X[16, 4, 17, 3], X[18, 9, 19, 10], X[14, 7, 15, 8], X[20, 13, 1, 14], X[8, 17, 9, 18], X[10, 19, 11, 20], X[12, 6, 13, 5], X[4, 12, 5, 11], X[2, 16, 3, 15]].

| Homological Grading $r$ | Quantum Grading $q$ | Spectra $S_L^{r,q}$ |
|---|---|---|
| -5 | -11 | 0 |

| | | |
|---|---|---|
| -5 | -9 | 0.697224, 1.11826, 2.59669, 3.26234, 4.30278, 8.02271 |
| -5 | -7 | 2.03698, 2.08531, 2.93548, 3.15866, 3.88992, 4.25586, 5.42973, 5.8209, 6.32086, 6.47383, 7.30709, 8.32802, 9.20254, 10.3506, 12.4042 |
| -5 | -5 | 3.3907, 3.52179, 4.32275, 5.02489, 5.07514, 5.89611, 6.10925, 6.48686, 7.11891, 7.60851, 8, 8.06526, 9.12384, 9.22948, 10.0933, 10.2648, 11.1606, 12.2729, 12.4128, 14.8221 |
| -5 | -3 | 4.89543, 5.63696, 6.42839, 6.92978, 7.62687, 7.79255, 8.55563, 9.66683, 9.69871, 10.0755, 10.5152, 11.0919, 12.6637, 13.2357, 15.1869 |
| -5 | -1 | 7, 8.38197, 9.20871, 10.618, 11, 13.7913 |
| -5 | 1 | 10 |
| -4 | -9 | 0, 0, 0.697224, 1.11826, 2, 2, 2.59669, 3.26234, 4.30278, 8.02271 |
| -4 | -7 | 0, 0.729232, 0.948606, 1.1296, 2.03698, 2.08531, 2.20434, 2.60347, 2.60347, 2.84943, 2.93111, 2.93548, 3.15866, 3.28654, 3.52866, 3.78146, 3.88992, 3.98904, 4, 4, 4.25586, 4.64671, 4.76346, 4.86898, 4.86898 |

| | | |
|---|---|---|
| -4 | -5 | 0.957766, 1.88024, 2.4249, 2.43012, 2.61585, 3.08718, 3.26397, 3.3907, 3.52179, 3.53737, 3.90303, 4.07778, 4.1089, 4.1089, 4.18488, 4.21819, 4.32275, 4.65921, 4.65921, 4.86168, 5.00645, 5.02489, 5.07514, 5.11125, 5.20443 |
| -4 | -3 | 2.60685, 3.65364, 3.97573, 4.22971, 4.30619, 4.75926, 4.89543, 5.17296, 5.18983, 5.56598, 5.63696, 5.87804, 5.89064, 5.89064, 5.98065, 6.20723, 6.35947, 6.42839, 6.50233, 6.70437, 6.70437, 6.71421, 6.92978, 6.94991, 7.09091 |
| -4 | -1 | 5.19321, 6.10578, 6.46235, 6.66807, 6.70875, 7, 7.04046, 7.73028, 7.91661, 8.01943, 8.01943, 8.38197, 8.41951, 8.52515, 9.01967, 9.15682, 9.19183, 9.20871, 9.33421, 9.43763, 10.0387, 10.2801, 10.4026, 10.4968, 10.5362 |
| -4 | 1 | 10, 10, 10, 10, 10, 10, 10, 10, 12, 12 |
| -3 | -9 | 2, 2 |
| -3 | -7 | 0, 0, 0, 0, 0.729232, 0.948606, 1.1296, 2, 2, 2.20434, 2.4576, 2.4576, 2.60347, 2.60347, 2.84943, 2.93111, 3.28654, 3.52866, 3.75996, 3.75996, 3.78146, 3.98904, 4, 4, 4 |

| | | |
|---|---|---|
| -3 | -5 | 0, 0, 0.432352, 0.432352, 0.957766, 1.37277, 1.37277, 1.88024, 1.95444, 2.27551, 2.27551, 2.3203, 2.4249, 2.43012, 2.47733, 2.61585, 2.93873, 2.93873, 3.08718, 3.24598, 3.26397, 3.40452, 3.40452, 3.53737, 3.76562 |
| -3 | -3 | 1.00399, 1.46315, 1.46315, 1.79299, 1.93165, 2.55506, 2.55506, 2.60685, 2.75636, 2.98722, 2.98722, 3.44264, 3.6017, 3.6017, 3.65364, 3.92207, 3.97573, 4.06808, 4.06808, 4.07768, 4.22971, 4.23518, 4.24006, 4.24006, 4.27227 |
| -3 | -1 | 2.88406, 3.165, 3.165, 3.88189, 3.88189, 4.77287, 4.79735, 4.79735, 4.92118, 5.0161, 5.19321, 5.39016, 5.39016, 5.77842, 5.77842, 5.78835, 5.81336, 6.02909, 6.10578, 6.12667, 6.12667, 6.42505, 6.42505, 6.45703, 6.46235 |
| -3 | 1 | 5.35024, 5.35024, 6.13025, 6.13025, 7.2901, 7.2901, 8.53014, 8.53014, 9.48233, 9.48233, 10, 10, 10, 10, 10, 10, 10, 10, 10, 10, 10, 10, 10, 10, 10 |
| -3 | 3 | 8, 8 |
| -2 | -7 | 2, 2, 2.4576, 2.4576, 3.75996, 3.75996, 4, 4, 4, 4, 4, 4, 4, 4, 4.74276, 4.74276, 5.25786, 5.25786, 9.78182, 9.78182 |

| | | |
|---|---|---|
| -2 | -5 | 0, 0, 0, 0, 0, 0, 0.432352, 0.432352, 1.37277, 1.37277, 1.46959, 1.86172, 1.86172, 1.95444, 2, 2, 2.27551, 2.27551, 2.3203, 2.47733, 2.69583, 2.93873, 2.93873, 3.01491, 3.01491 |
| -2 | -3 | 0, 0, 0, 0, 0.326251, 0.326251, 1.00399, 1.23738, 1.23738, 1.46315, 1.46315, 1.64505, 1.64505, 1.79299, 1.93165, 1.97968, 1.97968, 1.99759, 1.99759, 2.18025, 2.18025, 2.42531, 2.46784, 2.46784, 2.55012 |
| -2 | -1 | 0.942193, 0.942193, 1.40231, 1.40231, 2.38779, 2.38779, 2.70889, 2.70889, 2.7309, 2.88406, 2.89691, 2.93393, 2.93393, 2.98512, 3.165, 3.165, 3.20097, 3.20097, 3.52568, 3.54583, 3.54583, 3.79342, 3.79342, 3.88189, 3.88189 |
| -2 | 1 | 2.82504, 2.82504, 3.35083, 3.35083, 4.14954, 4.14954, 5.05365, 5.05365, 5.08924, 5.35024, 5.35024, 5.37025, 5.37025, 5.57749, 5.57749, 5.67252, 5.82027, 5.82027, 5.9125, 5.9125, 5.95426, 5.95426, 6.13025, 6.13025, 6.17264 |
| -2 | 3 | 7, 7, 7.43845, 7.43845, 8, 8, 8, 8, 8, 8, 8, 8, 8, 8, 8, 8, 8, 11.5616, 11.5616, 12 |
| -1 | -7 | 4, 4, 4 |

| | | |
|---|---|---|
| -1 | -5 | 1.46959, 1.86172, 1.86172, 2, 2, 2.69583, 3.01491, 3.01491, 3.65538, 3.65538, 4, 4, 4, 4, 4, 4, 4.24968, 4.24968, 4.5359, 4.55343, 4.55343, 4.58625, 4.58625, 4.7141, 5 |
| -1 | -3 | 0, 0, 0, 0, 0, 0, 0.326251, 0.326251, 1.23738, 1.23738, 1.64505, 1.64505, 1.75818, 1.75818, 1.86638, 1.89734, 1.90709, 1.97968, 1.97968, 1.99759, 1.99759, 2.18025, 2.18025, 2.42531, 2.46784 |
| -1 | -1 | 0, 0, 0, 0, 0, 0, 0.354247, 0.942193, 0.942193, 1.06092, 1.11966, 1.40231, 1.40231, 1.41337, 1.41337, 1.94372, 1.94372, 2.08653, 2.08653, 2.20644, 2.29184, 2.37445, 2.37445, 2.38779, 2.38779 |
| -1 | 1 | 0.825256, 0.825256, 1.34245, 2.24177, 2.61869, 2.61869, 2.77639, 2.82504, 2.82504, 2.88479, 2.88479, 2.92364, 2.92364, 3.0759, 3.0759, 3.27132, 3.35083, 3.35083, 3.39373, 3.39373, 3.76845, 3.76845, 3.90797, 3.90797, 4.04114 |
| -1 | 3 | 2.62723, 2.62723, 2.88559, 4.46887, 4.89567, 4.89567, 5.93304, 6.12702, 6.37425, 6.37425, 6.61224, 6.61224, 7, 7, 7, 7, 7, 7, 7, 7, 7, 7, 7, 7.01065, 7.16779, 7.25834, 7.25834, 7.26249, 7.26249 |
| -1 | 5 | 6, 6, 6 |
| 0 | -5 | 4, 4, 4.5359, 5, 6, 6, 6.76393, 6.76393, 7, 7, 7, 7, 7, 7, 7, 7, 7, 7, 7, 7, 7, 7, 7, 7, 7 |

| | | |
|---|---|---|
| 0 | -3 | 1.75818, 1.75818, 1.86638, 1.89734, 1.90709, 2.5631, 3.14907, 3.14907, 3.24667, 3.26289, 3.55815, 3.56887, 3.56887, 3.59226, 3.61066, 3.75952, 3.8046, 4.07183, 4.12991, 4.29792, 4.33829, 4.49721, 4.55827, 4.55827, 4.66409 |
| 0 | -1 | 0, 0, 0, 0, 0, 0, 0, 0.354247, 1.06092, 1.11966, 1.41337, 1.41337, 1.50953, 1.58957, 1.8582, 1.91195, 1.94372, 1.94372, 1.94424, 2.04653, 2.08653, 2.08653, 2.20644, 2.29184, 2.37445 |
| 0 | 1 | 0, 0, 0, 0, 0, 0, 0, 0.825256, 0.825256, 1.07844, 1.08478, 1.22508, 1.34245, 1.38663, 1.39315, 1.45817, 1.45817, 2.1136, 2.1136, 2.166, 2.24177, 2.25588, 2.33298, 2.40099, 2.44052 |
| 0 | 3 | 1.24951, 2.12248, 2.48699, 2.5045, 2.61409, 2.62723, 2.62723, 2.65072, 2.65072, 2.67926, 2.73057, 2.74098, 2.88559, 2.94382, 2.94382, 3.4549, 3.51461, 3.81186, 3.99433, 4.01604, 4.24024, 4.32246, 4.33203, 4.36723, 4.46887 |
| 0 | 5 | 3, 4.16443, 4.18726, 5.10019, 5.15076, 5.44788, 6, 6, 6, 6, 6, 6, 6, 6, 6, 6, 6, 6, 6, 6.45665, 6.46418, 7.04079, 7.09719, 7.33666, 11.2096 |
| 1 | -5 | 7, 7, 7, 7, 7, 7, 7 |

| | | |
|---|---|---|
| 1 | -3 | 3.61066, 3.8046, 4.07183, 4.71796, 4.88382, 4.93829, 4.94368, 5.5592, 5.6061, 5.67916, 5.75991, 6, 6, 6.10819, 6.16292, 6.35539, 6.418, 6.54597, 6.60314, 6.63322, 6.76393, 6.83772, 6.83772, 6.83772, 6.83772 |
| 1 | -1 | 1.50953, 1.58957, 1.8582, 1.91195, 1.94424, 2.04653, 2.81562, 2.94833, 2.9903, 3.01462, 3.09864, 3.09864, 3.1283, 3.22062, 3.33876, 3.5248, 3.54531, 3.80266, 3.80681, 3.93744, 3.96792, 4.12103, 4.12723, 4.2004, 4.26677 |
| 1 | 1 | 0, 0, 0, 0, 0, 0, 1.07844, 1.08478, 1.22508, 1.38663, 1.39315, 1.42018, 1.45817, 1.45817, 1.67828, 1.94322, 1.95716, 2.1136, 2.1136, 2.166, 2.25588, 2.33298, 2.40099, 2.44052, 2.49305 |
| 1 | 3 | 0, 0, 0, 0, 0, 0, 1.09994, 1.13598, 1.179, 1.24951, 1.25239, 1.39823, 1.4263, 1.5472, 1.997, 2.00153, 2.05603, 2.08325, 2.12248, 2.19058, 2.23301, 2.23381, 2.48699, 2.5045, 2.61409 |
| 1 | 5 | 1.28095, 1.29447, 2.34637, 2.60702, 2.61103, 2.61449, 2.70932, 3, 3, 3, 3, 3.67273, 3.9258, 4.00928, 4.16443, 4.16443, 4.18726, 4.18726, 4.21743, 4.2175, 4.33431, 4.39445, 4.41118, 4.44159, 5 |
| 1 | 7 | 3, 3, 4, 4.23844, 5.63667, 6, 9.12489 |
| 2 | -5 | 7 |

| | | |
|---|---|---|
| 2 | -3 | 4.94368, 5.67916, 6.35539, 6.76393, 7, 8, 8, 8, 8, 8, 8, 8, 8, 8, 8, 8, 8, 8.20222, 8.2893, 8.47947, 9.37136, 11, 11, 11, 11 |
| 2 | -1 | 3.1283, 3.5248, 3.93744, 4.12103, 4.39581, 4.40164, 4.70641, 4.89699, 4.94081, 5.15313, 5.30128, 5.32439, 5.67928, 5.68268, 5.72657, 5.73361, 5.84796, 5.92946, 5.92998, 5.95468, 5.95607, 5.95607, 6.12033, 6.17633, 6.19545 |
| 2 | 1 | 1.42018, 1.67828, 1.94322, 1.95716, 2.5293, 2.63389, 2.64866, 2.71694, 2.74587, 2.74847, 3.04234, 3.0849, 3.3775, 3.38708, 3.3892, 3.52811, 3.57542, 3.6482, 3.69944, 3.72731, 3.74875, 3.74907, 3.84296, 3.85539, 3.86882 |
| 2 | 3 | 0, 0, 0, 0, 1.09994, 1.13598, 1.179, 1.25239, 1.28597, 1.28678, 1.39823, 1.4263, 1.5472, 1.997, 2.00153, 2.05603, 2.08325, 2.19058, 2.23301, 2.23381, 2.4182, 2.66438, 2.76512, 2.87978, 2.96366 |
| 2 | 5 | 0, 0, 0, 0, 0, 0, 1.07294, 1.28095, 1.29447, 1.37341, 1.65111, 1.65712, 1.96169, 2.13212, 2.34637, 2.51682, 2.60702, 2.61103, 2.61449, 2.70489, 2.70932, 2.96584, 2.97465, 3, 3 |
| 2 | 7 | 1.33784, 2.55142, 3, 3, 3, 3, 3, 3, 3, 4, 4, 4, 4, 4.23844, 4.23844, 4.29363, 4.43239, 5.63667, 5.63667, 5.85682, 6, 6, 6, 6, 6.19356 |
| 2 | 9 | 3 |

| | | |
|---|---|---|
| 3 | -3 | 8, 8, 11 |
| 3 | -1 | 5.95607, 5.95607, 6.17633, 6.77408, 6.97696, 7.57427, 8.0161, 8.0161, 8.1877, 9.33395, 9.38197, 9.97378, 10, 10, 10, 10, 10, 10, 10, 10, 10, 10, 10, 10, 10 |
| 3 | 1 | 3.74875, 3.74907, 4.01074, 4.33727, 4.35298, 4.81318, 4.87688, 5.18105, 5.49393, 5.60232, 5.61185, 5.7409, 5.82349, 5.83244, 5.88637, 6.02965, 6.06426, 6.08819, 6.17119, 6.17653, 6.19072, 6.25175, 6.25808, 6.29079, 6.41413 |
| 3 | 3 | 1.28597, 1.28678, 2.4182, 2.75718, 2.76512, 2.97021, 3.02981, 3.33802, 3.33891, 3.346, 3.38944, 3.40889, 3.52641, 3.62354, 3.6884, 3.81857, 3.90937, 3.94887, 4.12642, 4.13956, 4.29055, 4.30348, 4.35398, 4.54705, 4.5946 |
| 3 | 5 | 0, 0, 1.07294, 1.09542, 1.37341, 1.59121, 1.65111, 1.65712, 1.96169, 2.13212, 2.43137, 2.47507, 2.51682, 2.70489, 2.77494, 2.93236, 2.96584, 2.97465, 3.0432, 3.16002, 3.18909, 3.53321, 3.53813, 3.63761, 3.7458 |
| 3 | 7 | 0, 0, 0, 0, 0.787855, 0.789212, 1.33784, 2.1203, 2.53759, 2.55142, 3, 3, 3, 3, 3, 3.03219, 3.03987, 3.14796, 3.18762, 3.27208, 3.71134, 4, 4, 4, 4 |
| 3 | 9 | 3, 3, 3 |
| 4 | -1 | 10, 10, 10, 10, 10, 10, 10, 10, 13, 13 |

| | | |
|---|---|---|
| 4 | 1 | 5.49393, 6.08819, 6.25808, 6.29079, 6.35373, 6.4389, 6.57863, 8.21242, 8.38197, 8.4237, 8.65711, 8.69697, 8.70395, 9.22984, 9.22984, 9.39423, 9.55085, 9.77448, 9.91766, 9.98298, 10, 10.09, 10.2734, 10.3504, 10.48 |
| 4 | 3 | 2.75718, 3.62354, 3.6884, 4.12642, 4.29055, 4.41914, 4.61817, 5.02425, 5.05504, 5.4525, 5.51229, 5.90503, 6.18912, 6.42886, 6.51611, 6.60414, 6.61866, 6.8122, 6.86171, 6.91973, 7, 7, 7, 7.19371, 7.23382 |
| 4 | 5 | 1.09542, 1.59121, 2.43137, 2.47507, 2.59883, 2.77494, 2.93236, 3.24705, 3.92848, 4.01, 4.03836, 4.07118, 4.20763, 4.25527, 4.40246, 4.67825, 4.72642, 4.87882, 4.87984, 5.10809, 5.17531, 5.31265, 5.31265, 5.39238, 5.46504 |
| 4 | 7 | 0, 0.787855, 0.789212, 1.31477, 1.91204, 2.1203, 2.53759, 2.79037, 3.03219, 3.03987, 3.14796, 3.18762, 3.27208, 3.36621, 3.71134, 3.75698, 4, 4, 4.24913, 4.32404, 4.37056, 4.45249, 4.45249, 4.79574, 4.83557 |
| 4 | 9 | 0, 0, 0.426647, 1, 2.88387, 3, 3, 3, 4.22463, 8.46486 |
| 5 | -1 | 10 |
| 5 | 1 | 6.35373, 8.38197, 9.91766, 10.618, 10.8613, 13.8673 |

| | | |
|---|---|---|
| 5 | 3 | 4.41914, 4.61817, 6.8122, 7, 7.23382, 7.96551, 8.31423, 9.65239, 9.89997, 10.0638, 11.1635, 11.715, 12.3842, 13.4766, 15.2815 |
| 5 | 5 | 2.59883, 3.24705, 4.03836, 4.72642, 4.87882, 5.46504, 6.25868, 6.87279, 7.17394, 7.49039, 7.57537, 8.43386, 9.09297, 9.5215, 10.0926, 11.0038, 11.2442, 12.279, 12.9491, 15.0573 |
| 5 | 7 | 1.31477, 1.91204, 2.79037, 3.36621, 3.75698, 4.37056, 4.79574, 5.73372, 6.25075, 6.46321, 7.36478, 8.91073, 9.47993, 10.7067, 12.7835 |
| 5 | 9 | 0.426647, 1, 2.88387, 3, 4.22463, 8.46486 |
| 5 | 11 | 0 |
